# Supplementary material for: Entropy-Guided Attention for Private LLMs
Source: arXiv:2501.03489 source file (2025-01-08)
Supplement: Supplementary file 1 [file 28_fig_appendix_iFFN_5L6L.tex]

\begin{figure} [htbp]
\centering
%\subfloat[Weight normalization in FFN]{\includegraphics[width=.5\textwidth]{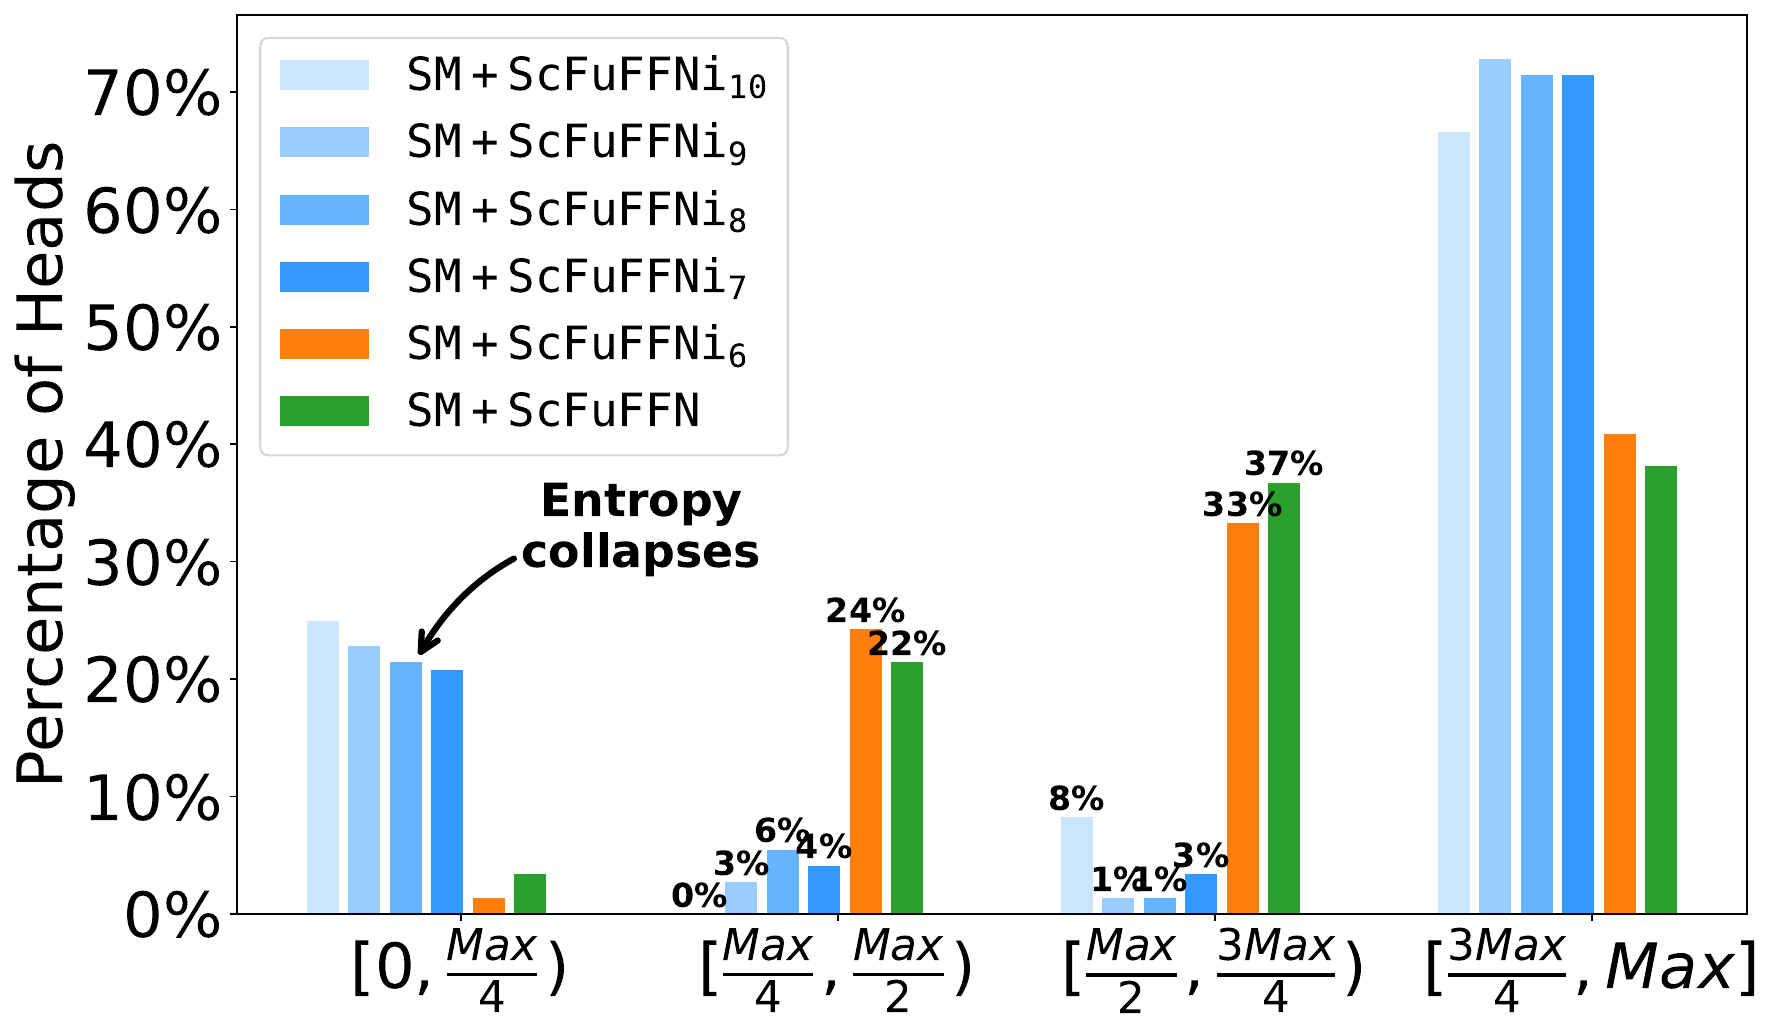}} 
\subfloat[Training instability (NaNs) in ${\tt SM+ScFuFFNi_7}$]{\includegraphics[width=.5\textwidth]{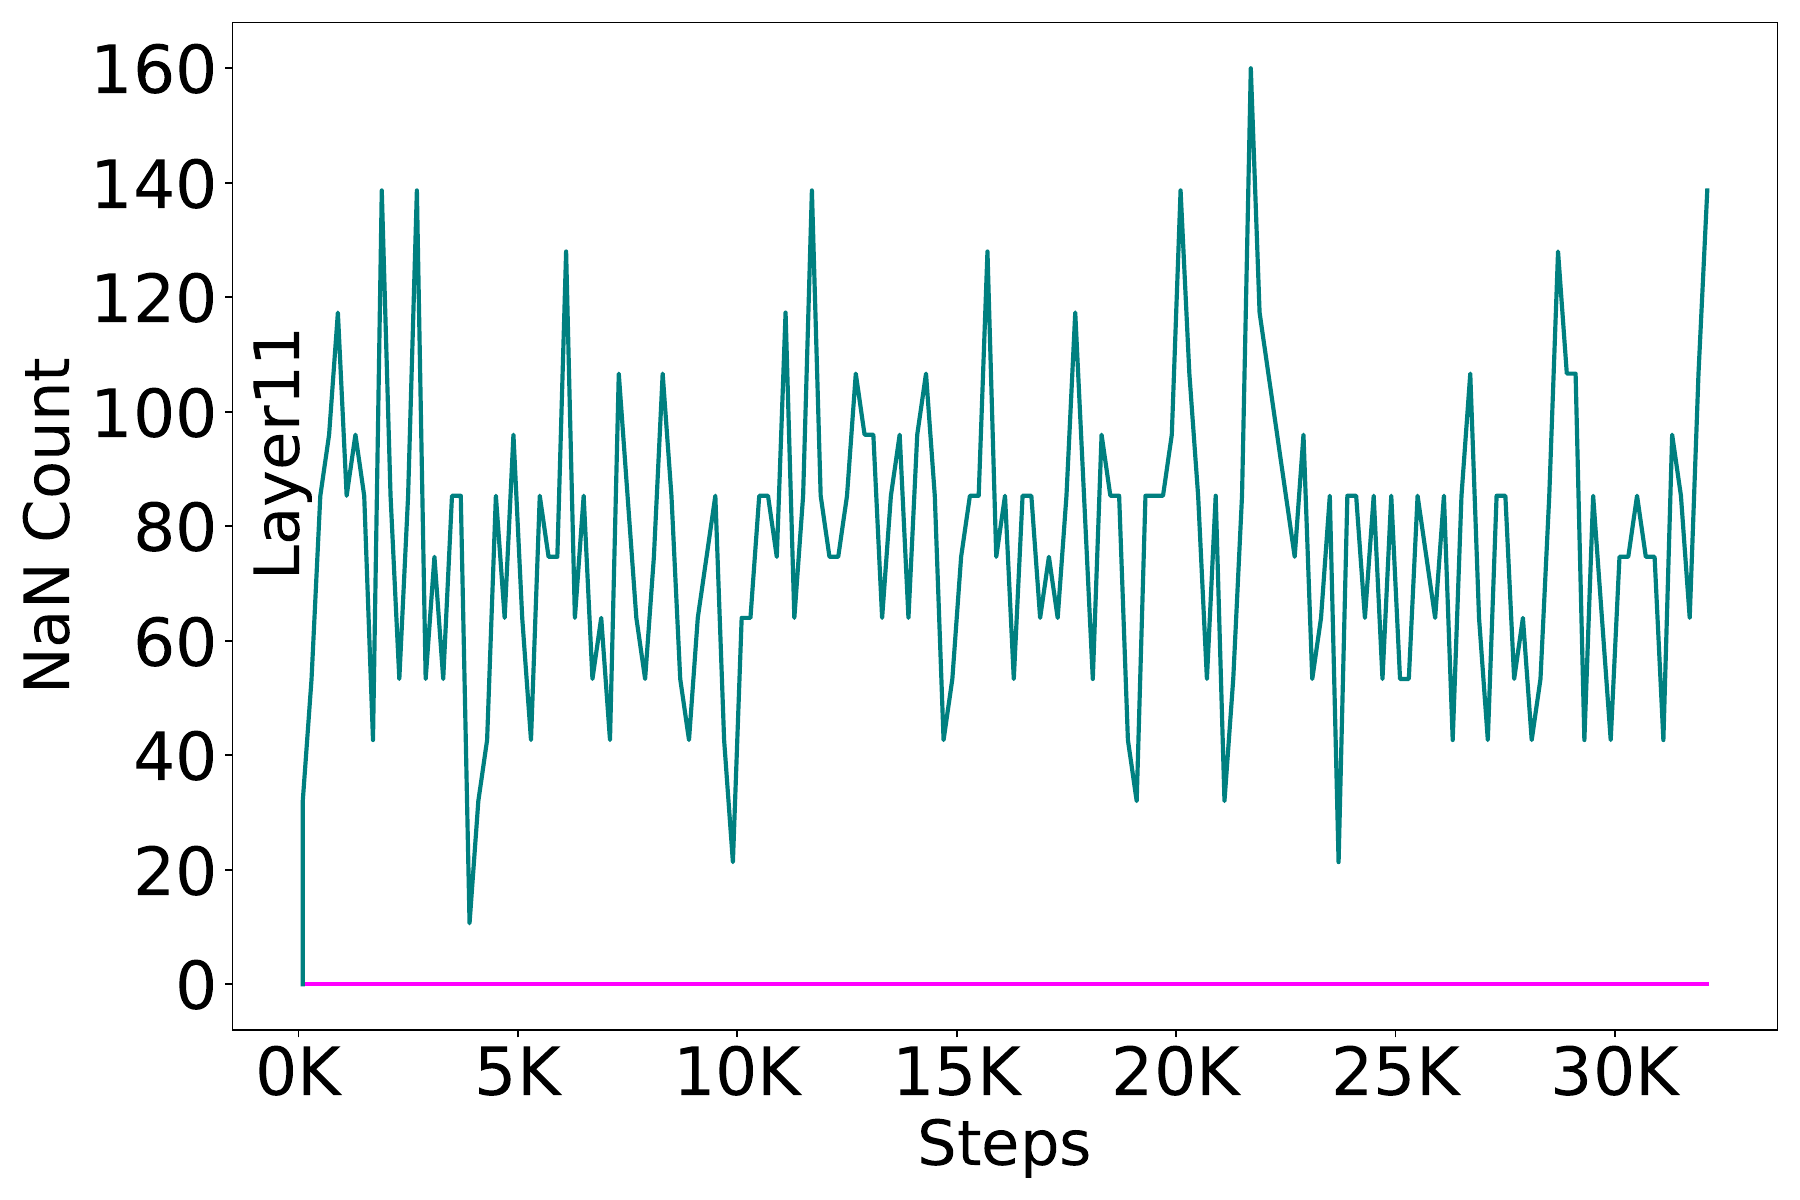}} 
\subfloat[Entropy collapses in ${\tt SM+ScFuFFNi_7}$ ]{\includegraphics[width=.5\textwidth]{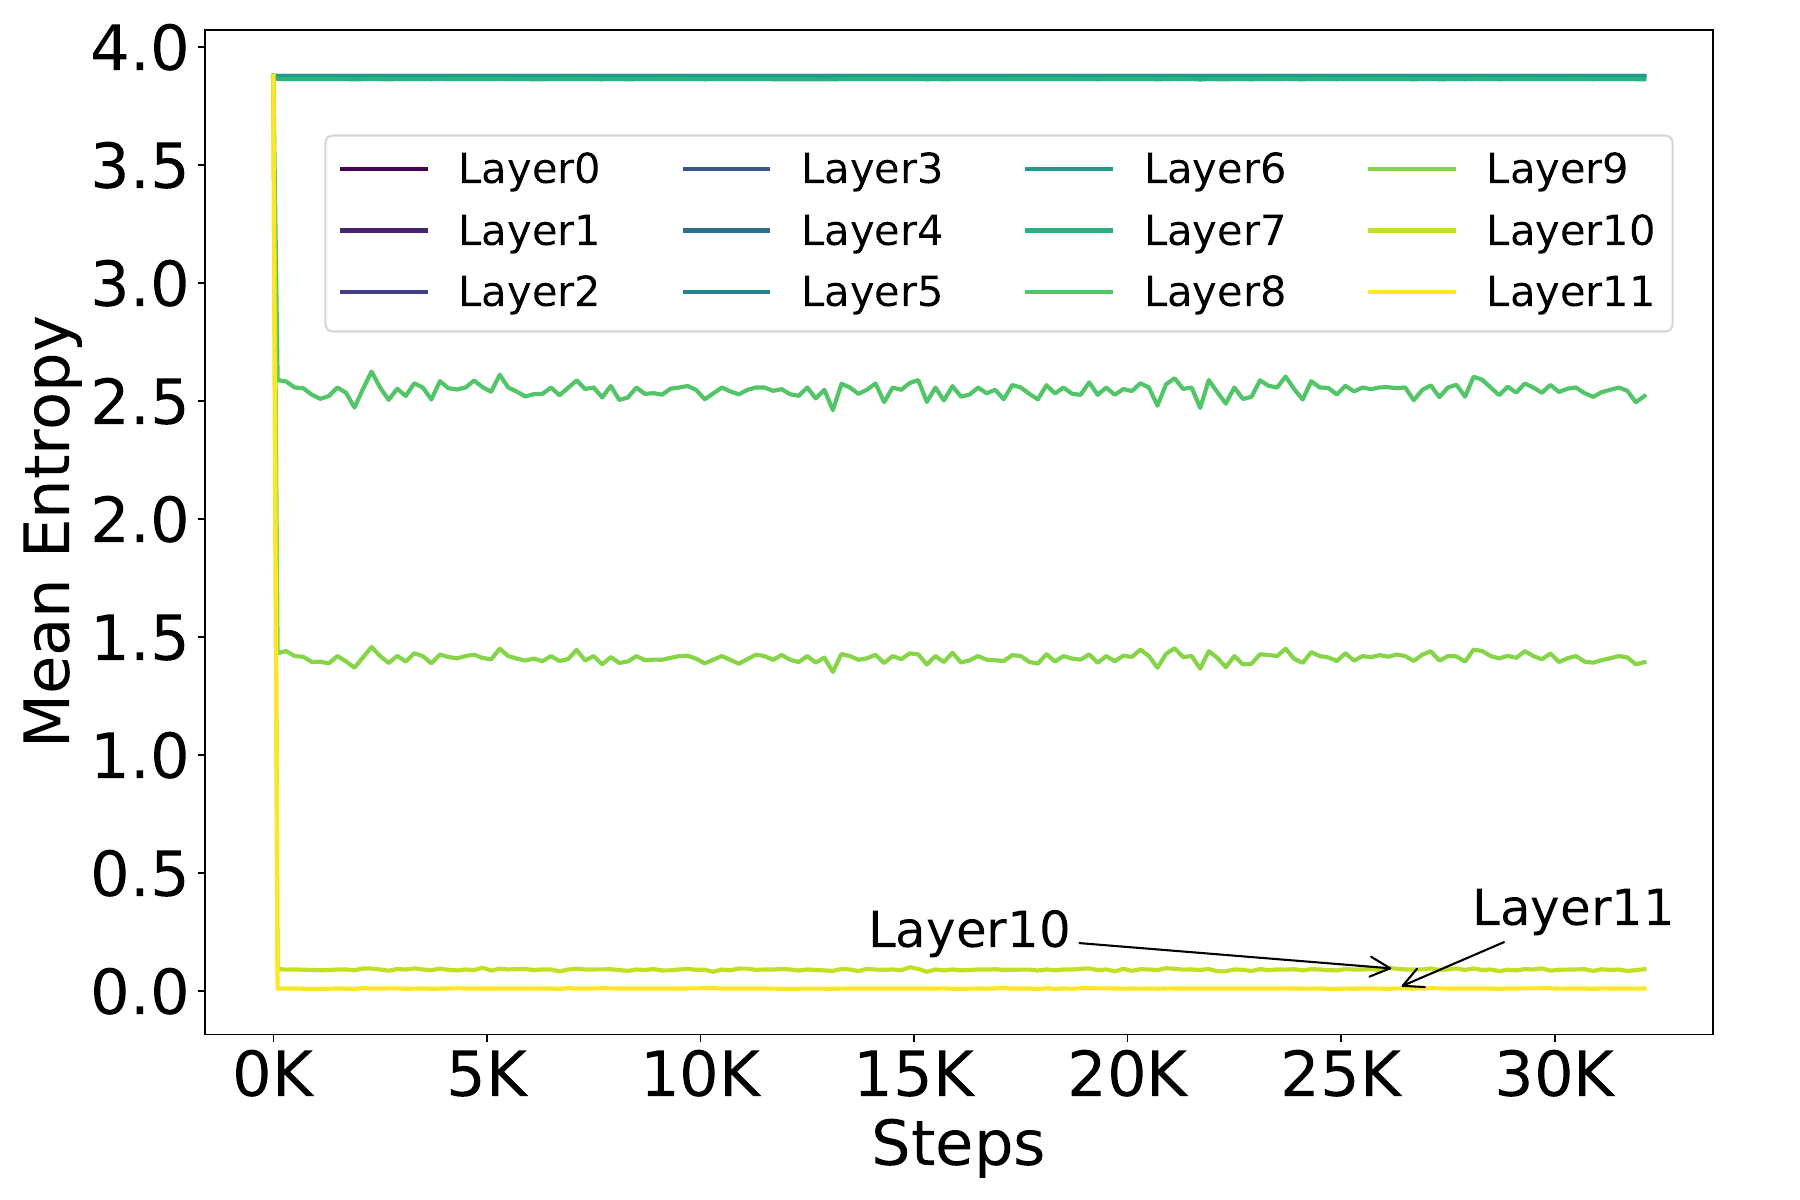}} \\  
\subfloat[Entropy dynamics in ${\tt SM+ScFuFFNi_6}$]{\includegraphics[width=.5\textwidth]{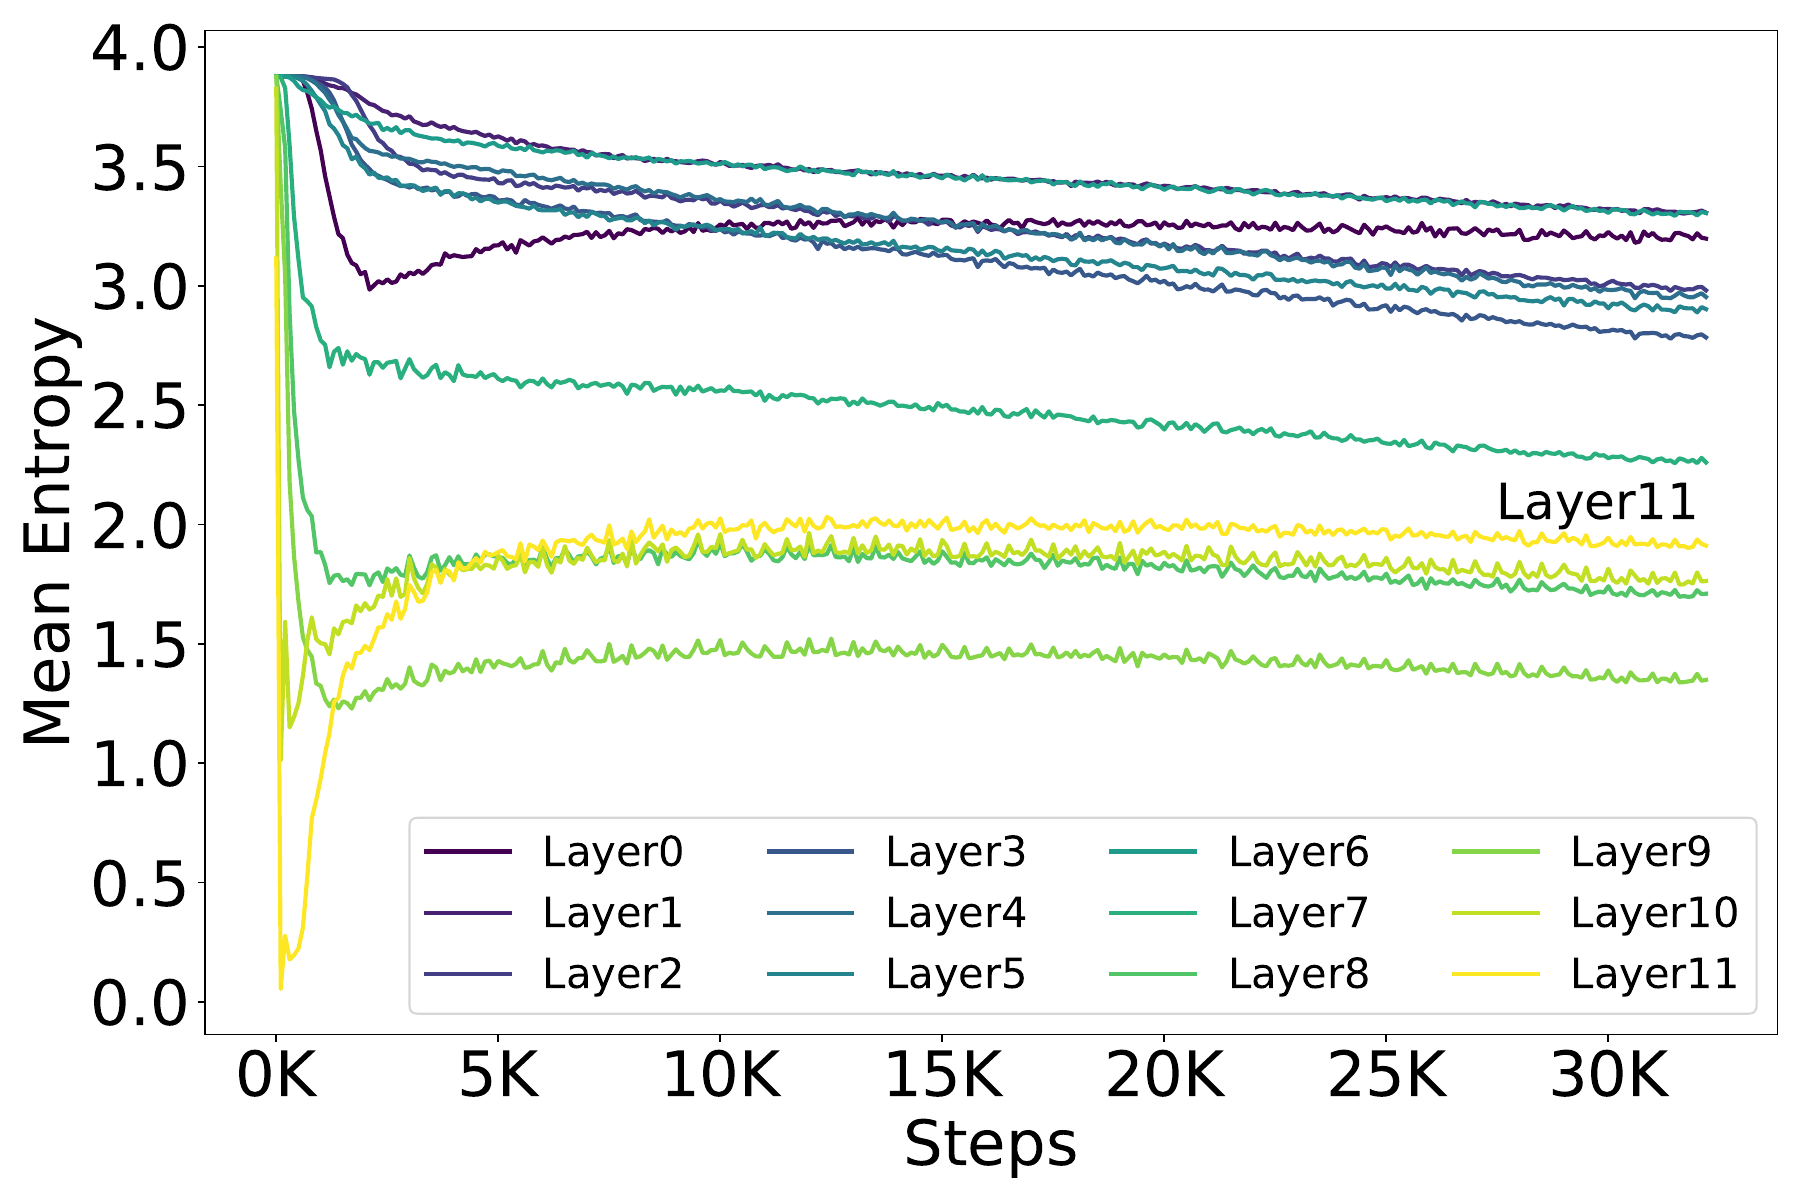}}  
\subfloat[Entropy dynamics in ${\tt SM+ScFuFFN}$]{\includegraphics[width=.5\textwidth]{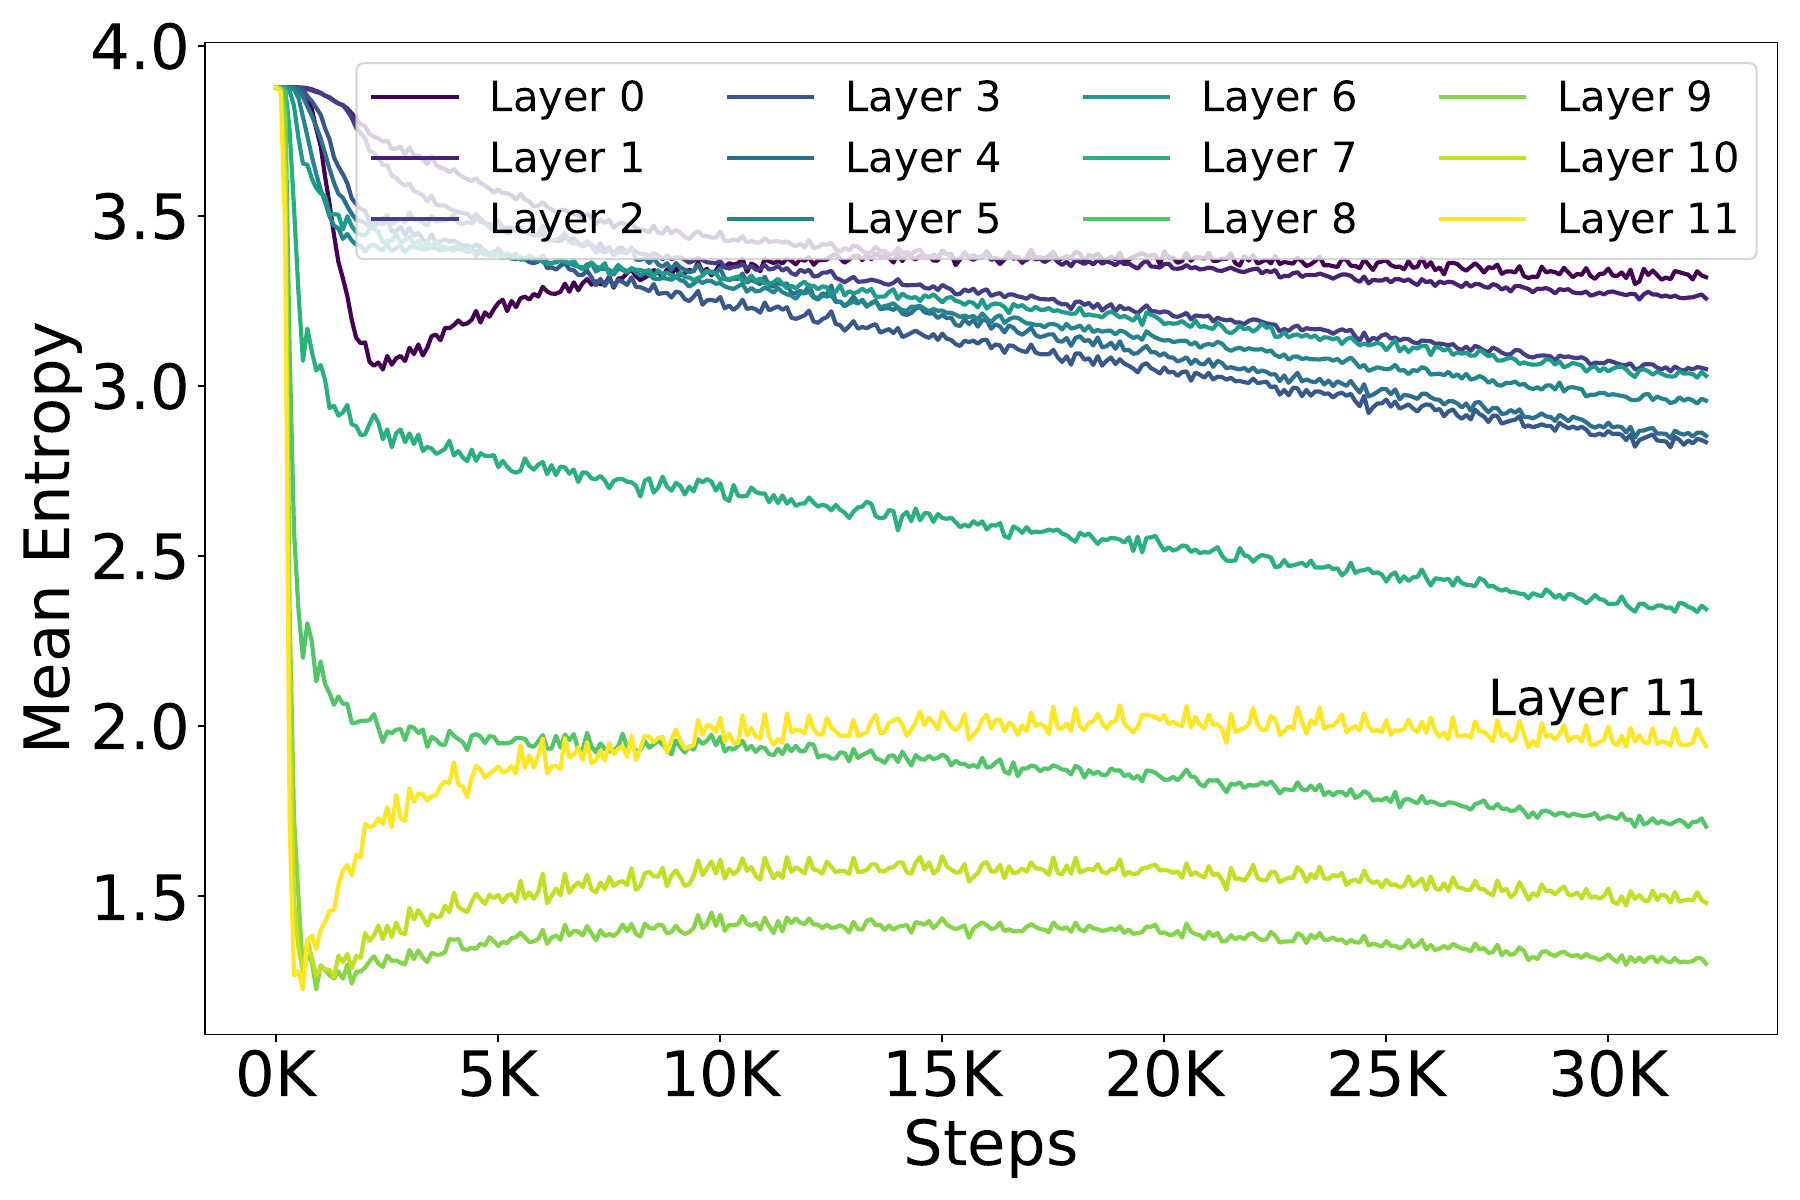}}  \\  \vspace{-0.5em}
\subfloat[${\tt SM+ScFuFFNi_7}$]{\includegraphics[width=.33\textwidth]{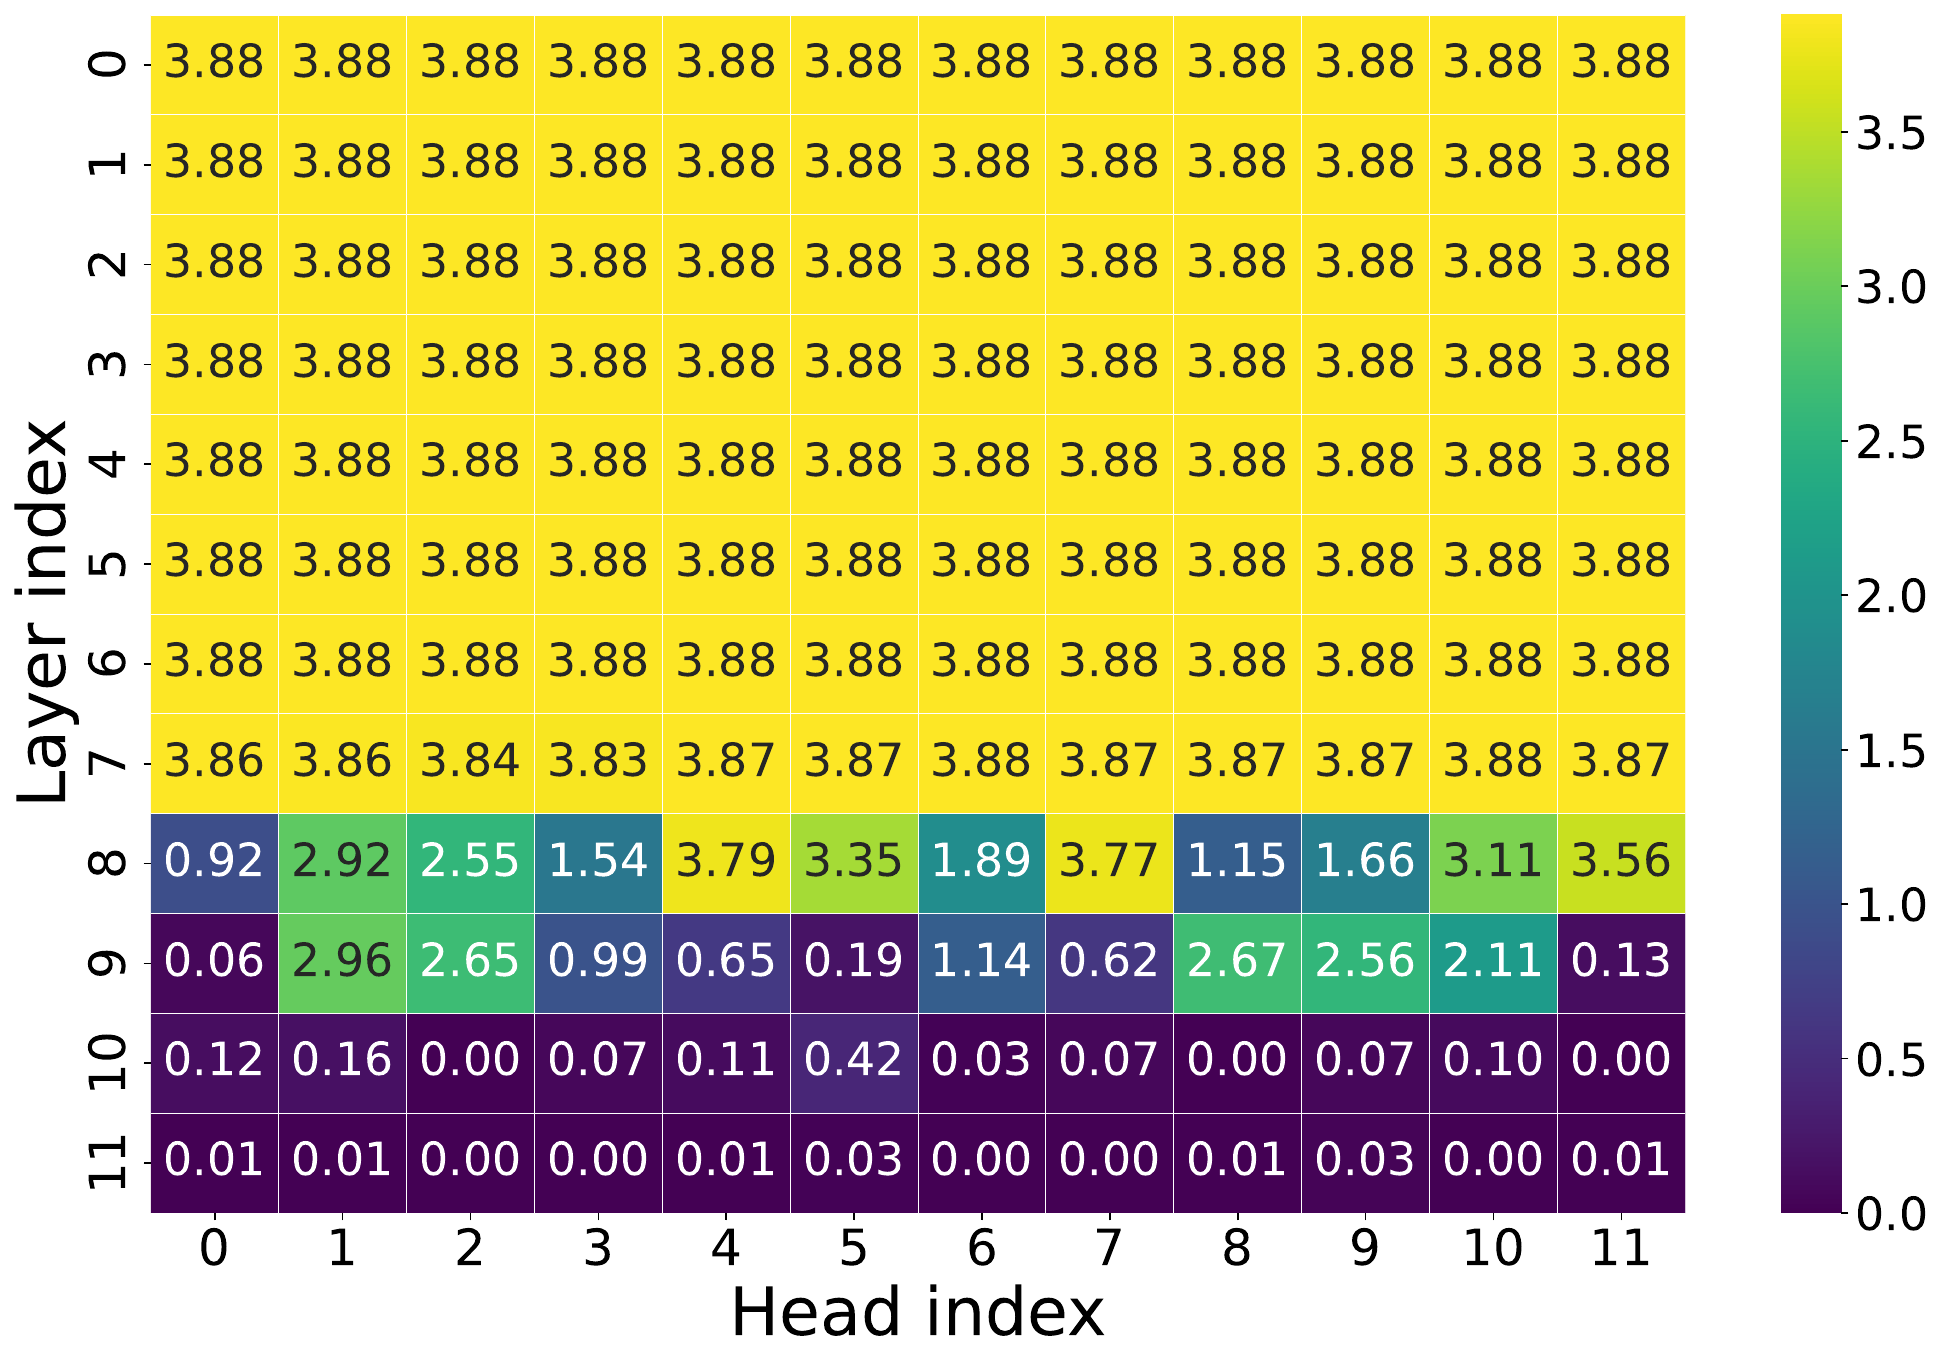}} 
\subfloat[${\tt SM+ScFuFFNi_6}$]{\includegraphics[width=.33\textwidth]{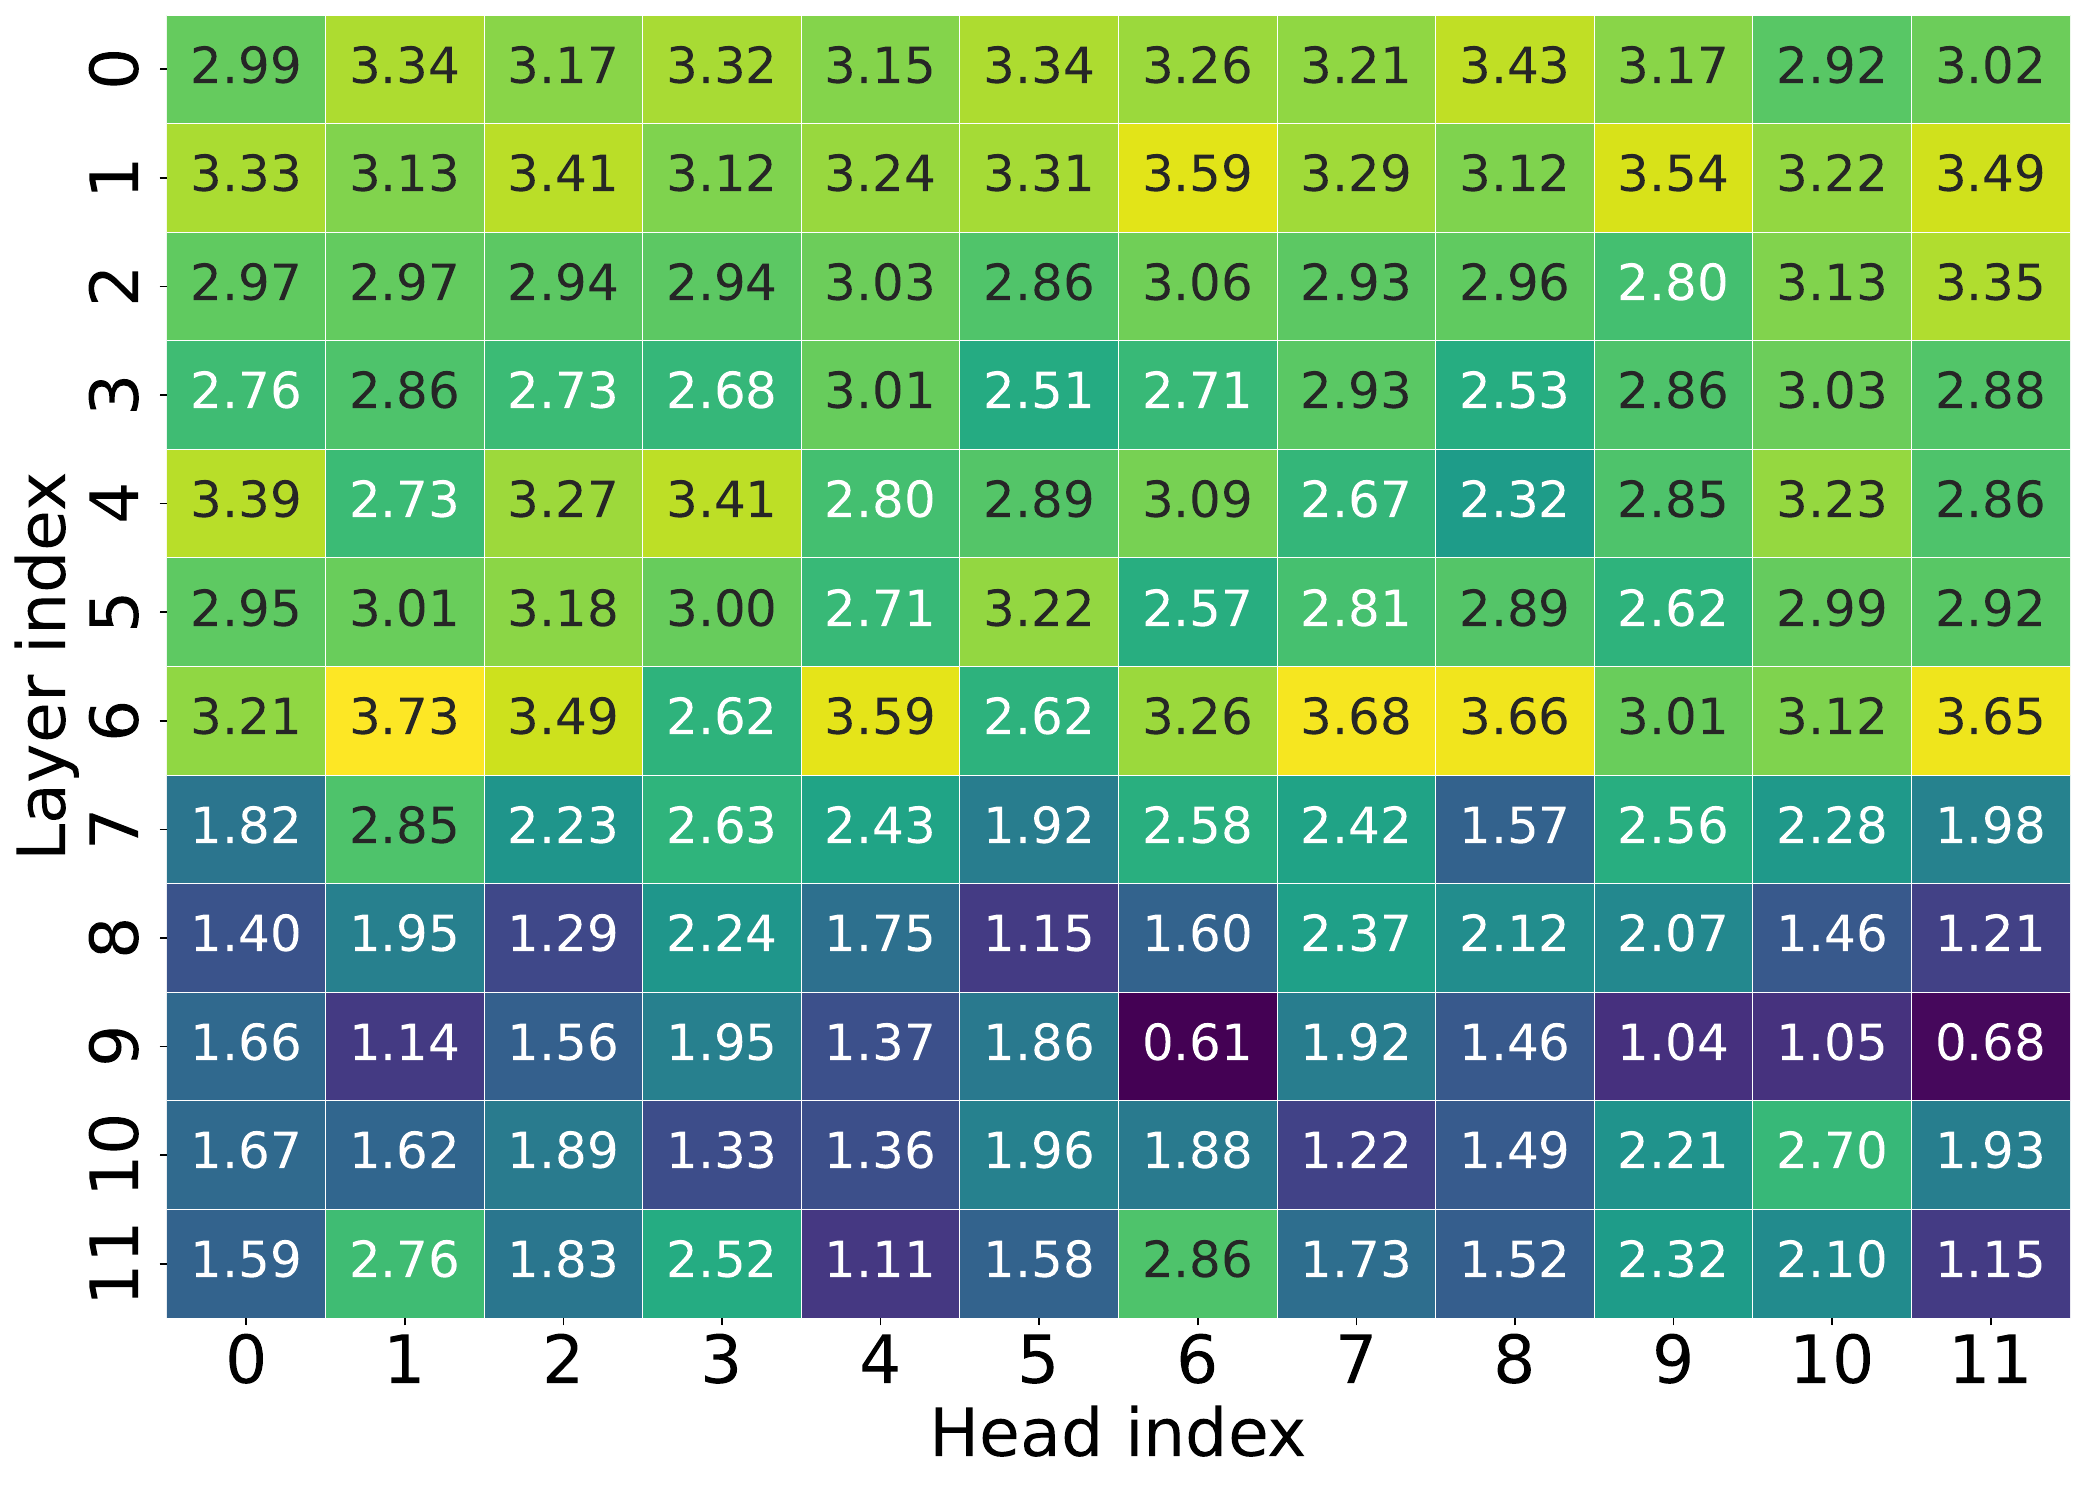}}  
\subfloat[${\tt SM+ScFuFFN}$]{\includegraphics[width=.33\textwidth]{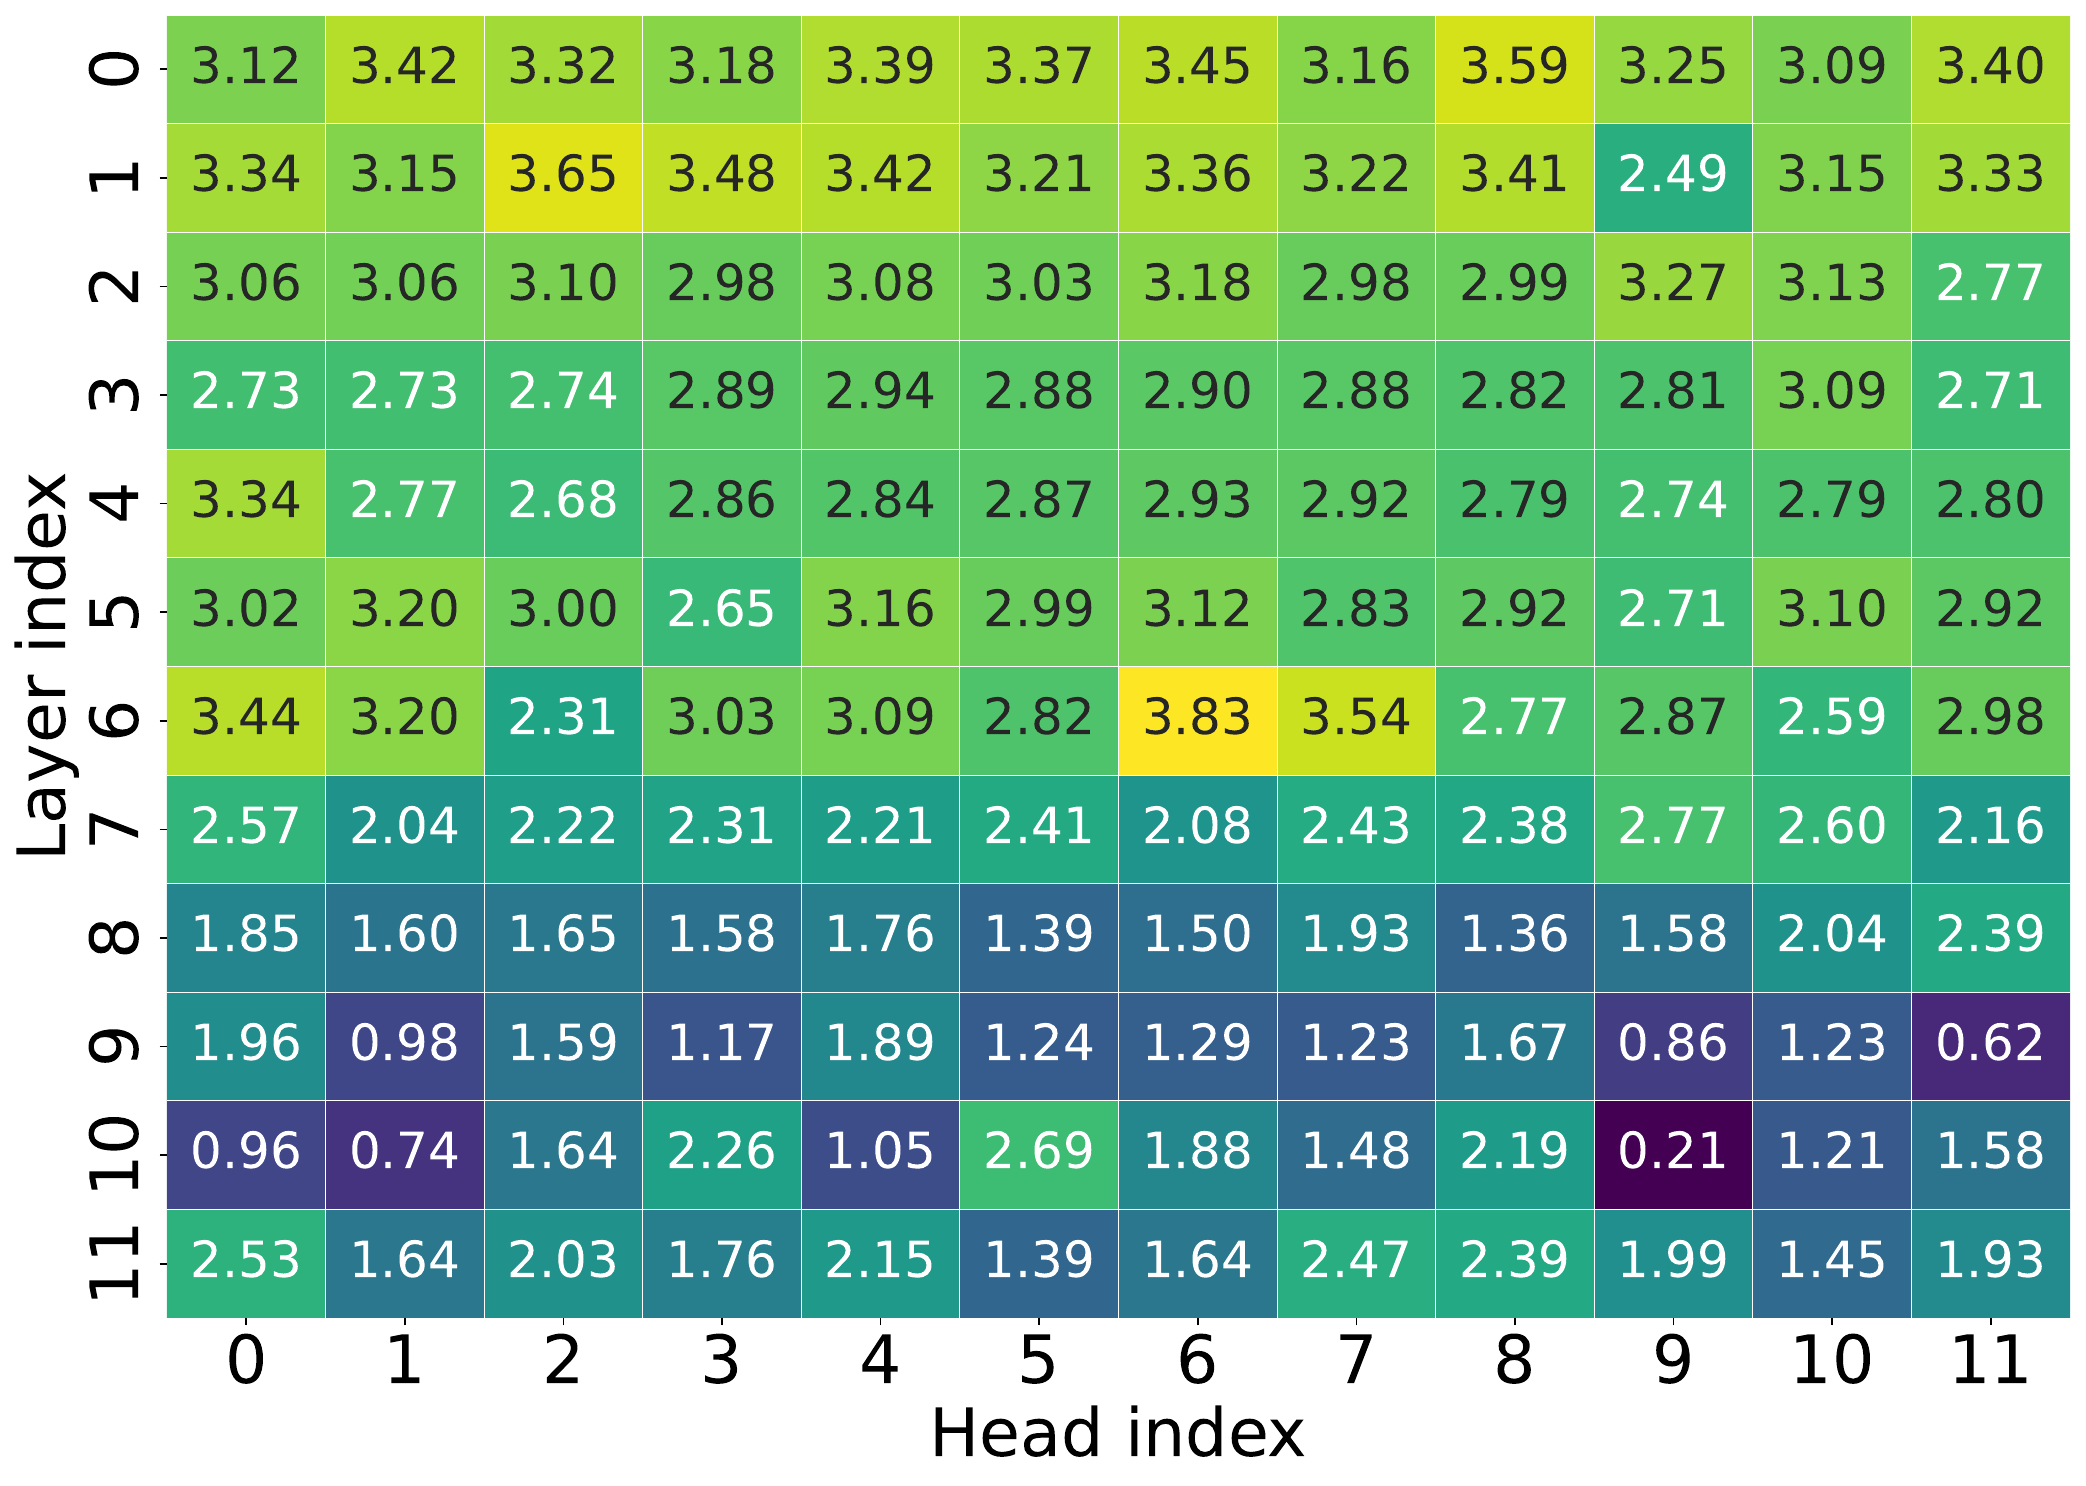}} \\ \vspace{-0.5em}
\caption{Training instability is evident with NaNs in the final layers (a) and entropy collapse in the last two layers (b) of the ${\tt SM+ScFuFFNi_7}$ configuration, where 7 deeper FFNs are pruned in the Softmax-only GPT-2 model ($L$ = 12, $H$ = 12, $d$ = 768), trained from scratch on the CodeParrot dataset. In contrast, stable training is observed in (c) with no entropy collapse when only 6 deeper FFNs are pruned (${ \tt SM+ScFuFFNi_6}$), and further validated against the unpruned configuration (${ \tt SM+ScFuFFN}$) in (d). The last row (e, f, g) shows entropy heatmaps for each configuration.}
\label{fig:TrainingDynamicsFFNi}
\end{figure}
