# Supplementary material for: Entropy-Guided Attention for Private LLMs
Source: arXiv:2501.03489 source file (2025-01-08)
Supplement: Supplementary file 2 [file 20_fig_appendix_layerwise_entropy.tex]

\begin{figure} [htbp]
\centering
\subfloat[SM + LN + G \label{subfig:sm_ln_g}]{\includegraphics[width=.5\textwidth]{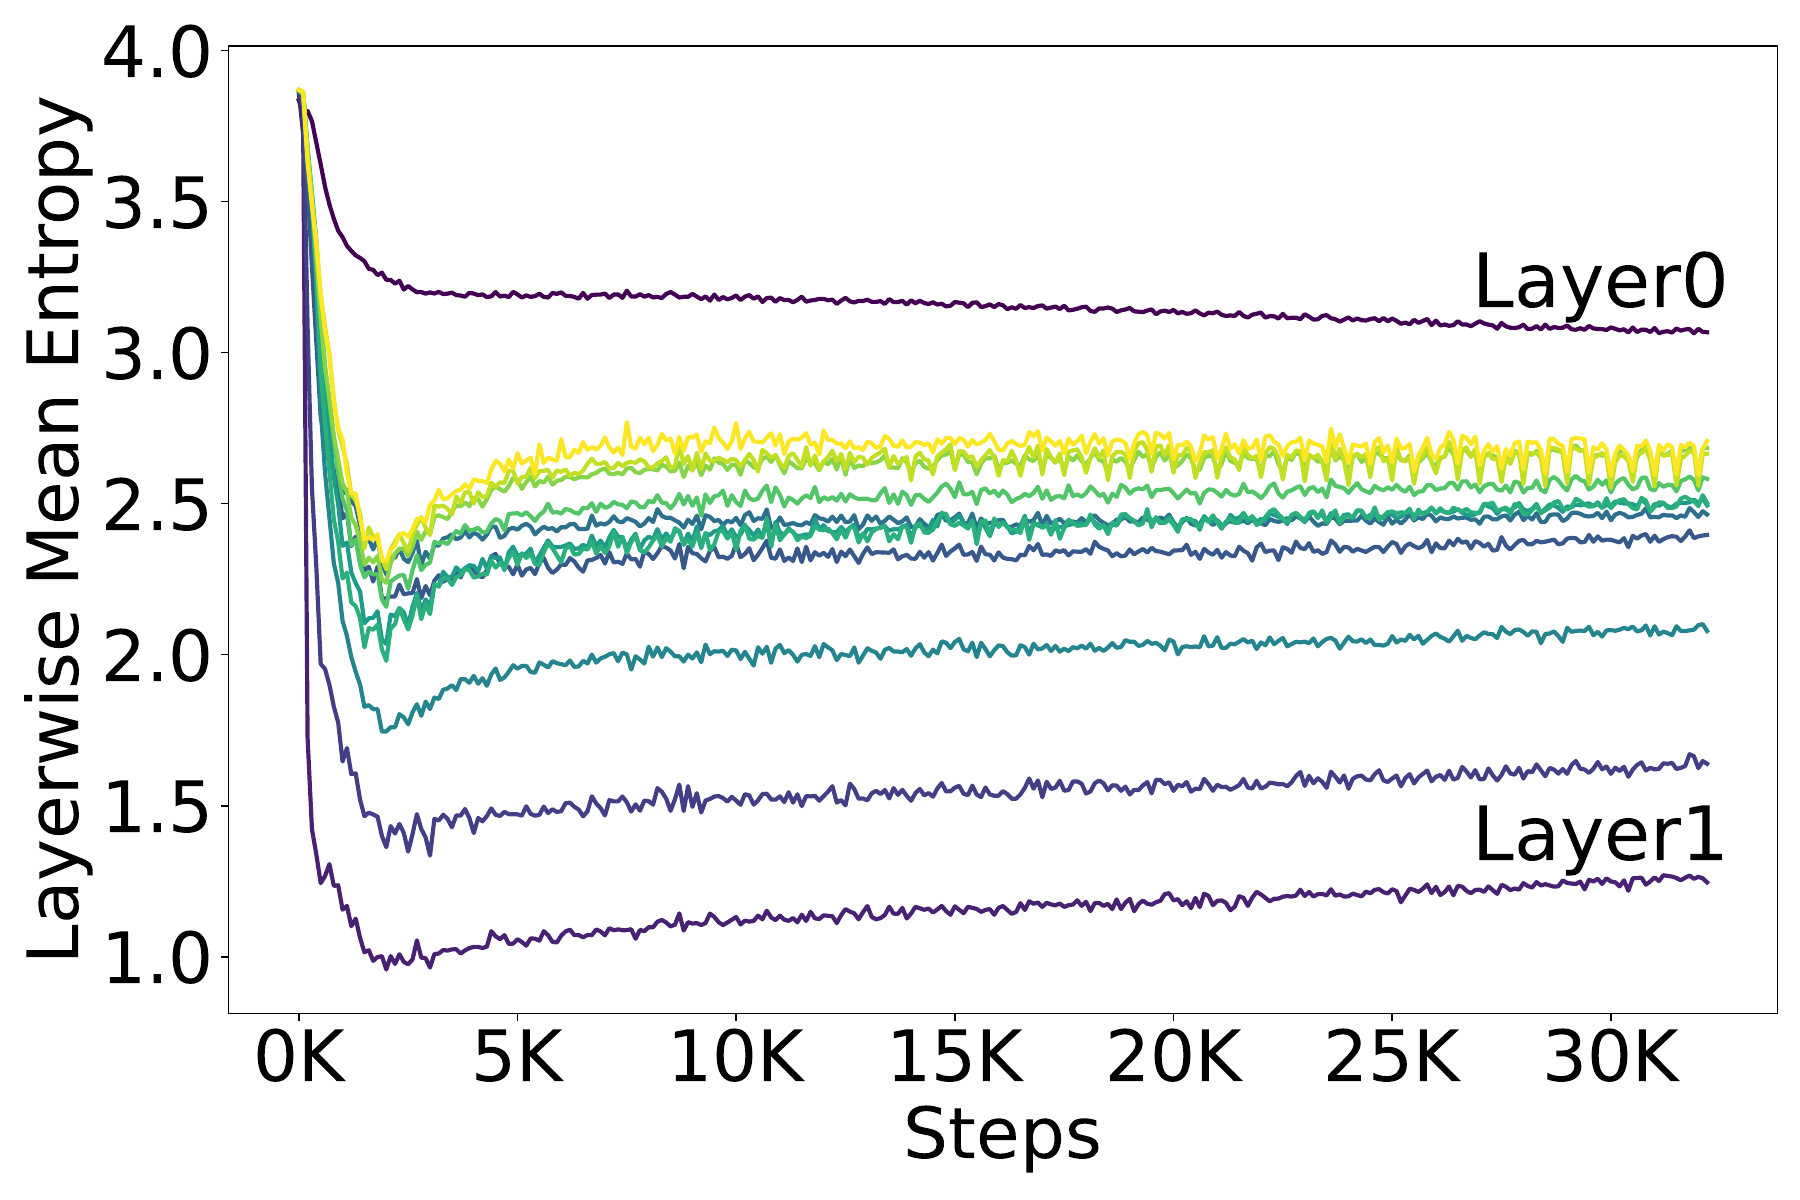}} 
\subfloat[SM + LN + R \label{subfig:sm_ln_r}]{\includegraphics[width=.5\textwidth]{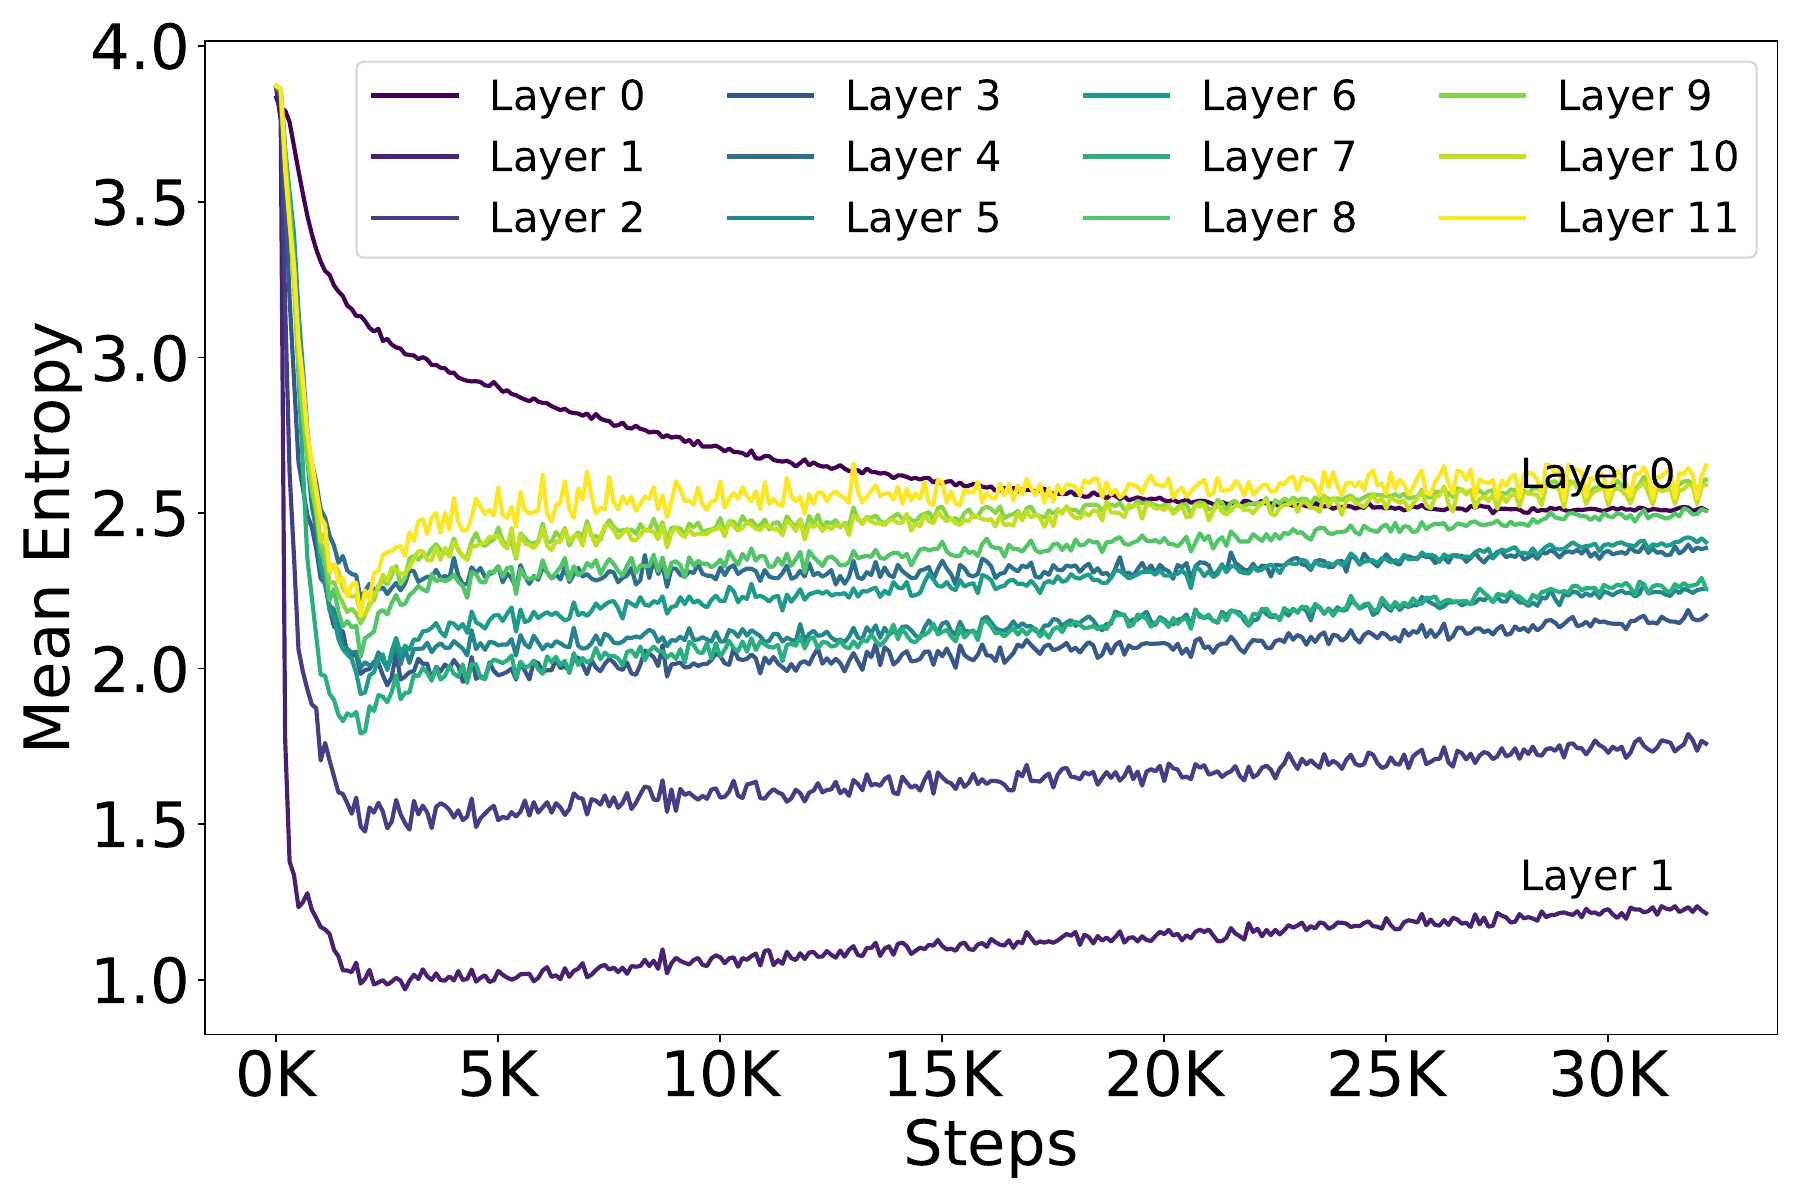}} \\
\subfloat[SM + LN ]{\includegraphics[width=.49\textwidth]{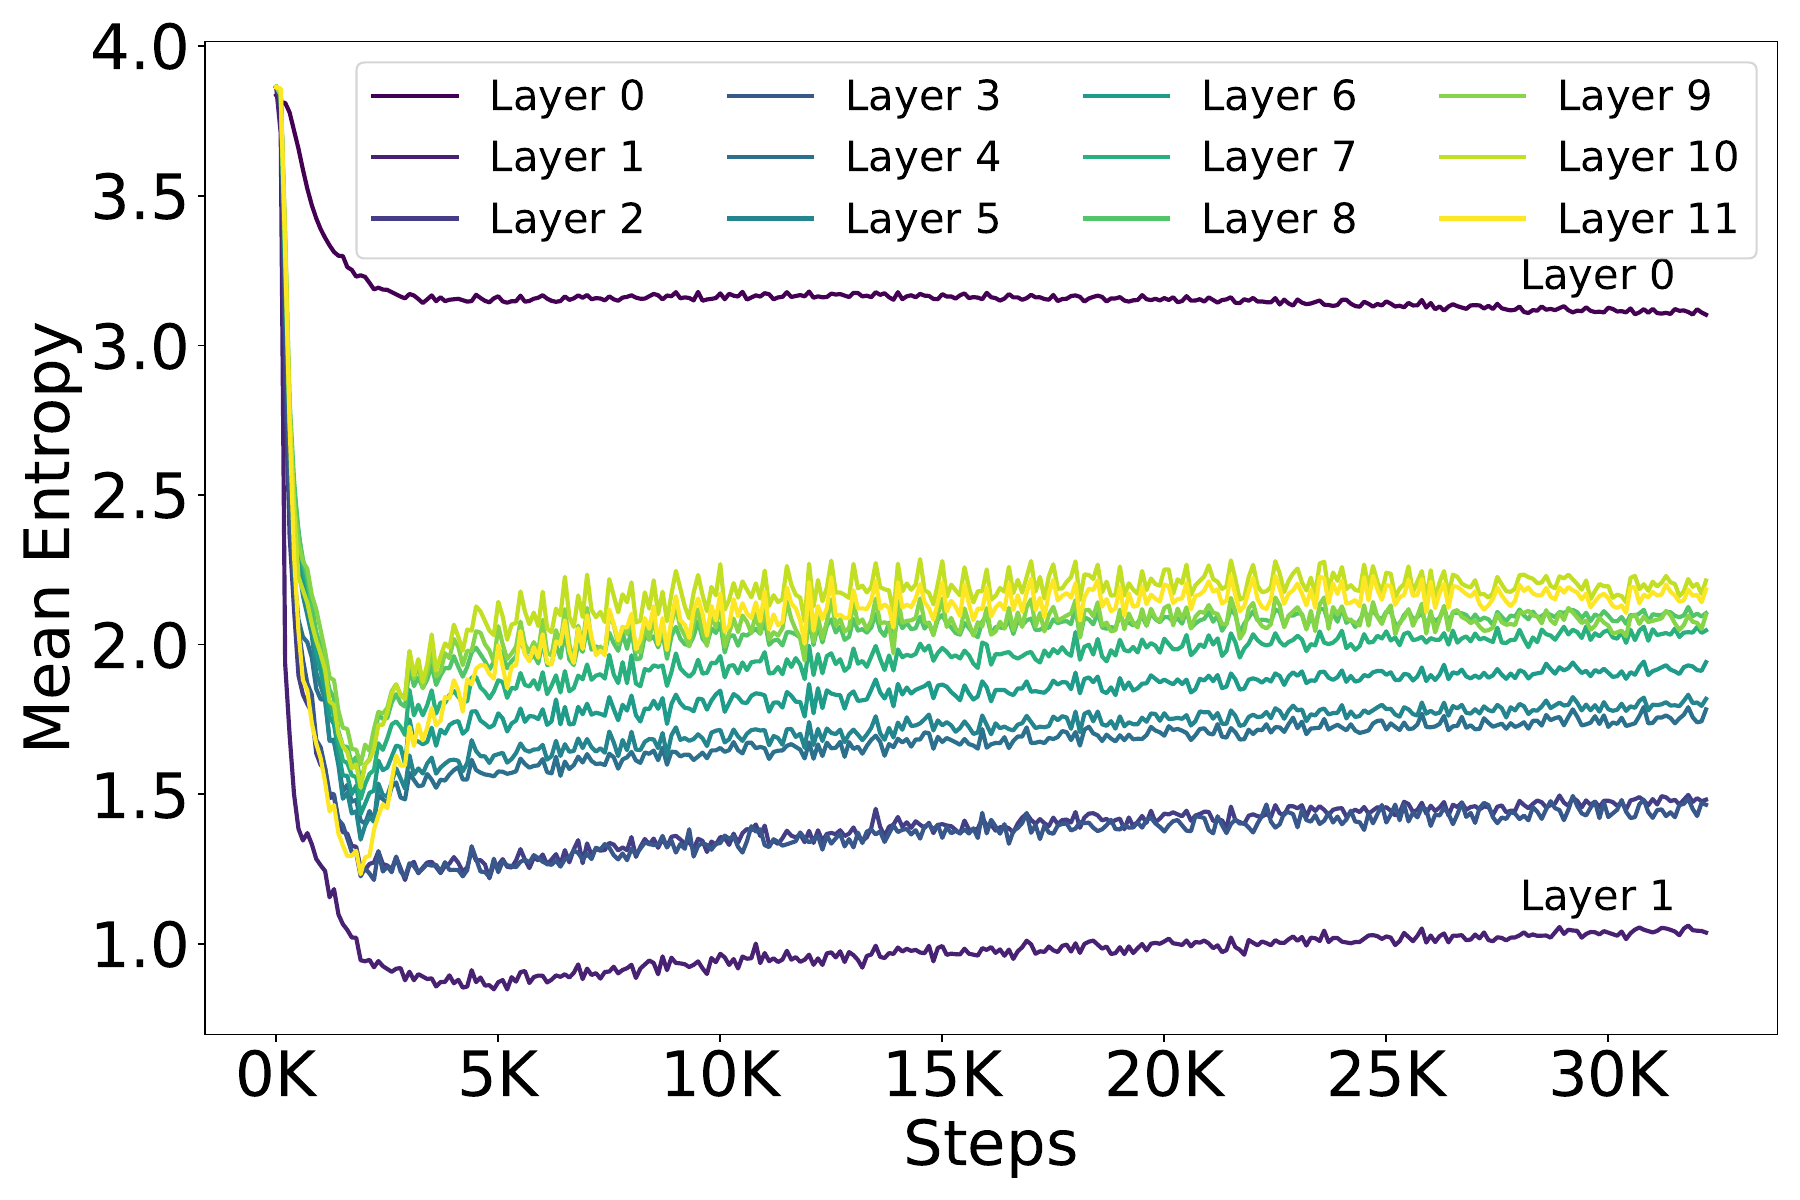}}  
\subfloat[SM + G]{\includegraphics[width=.49\textwidth]{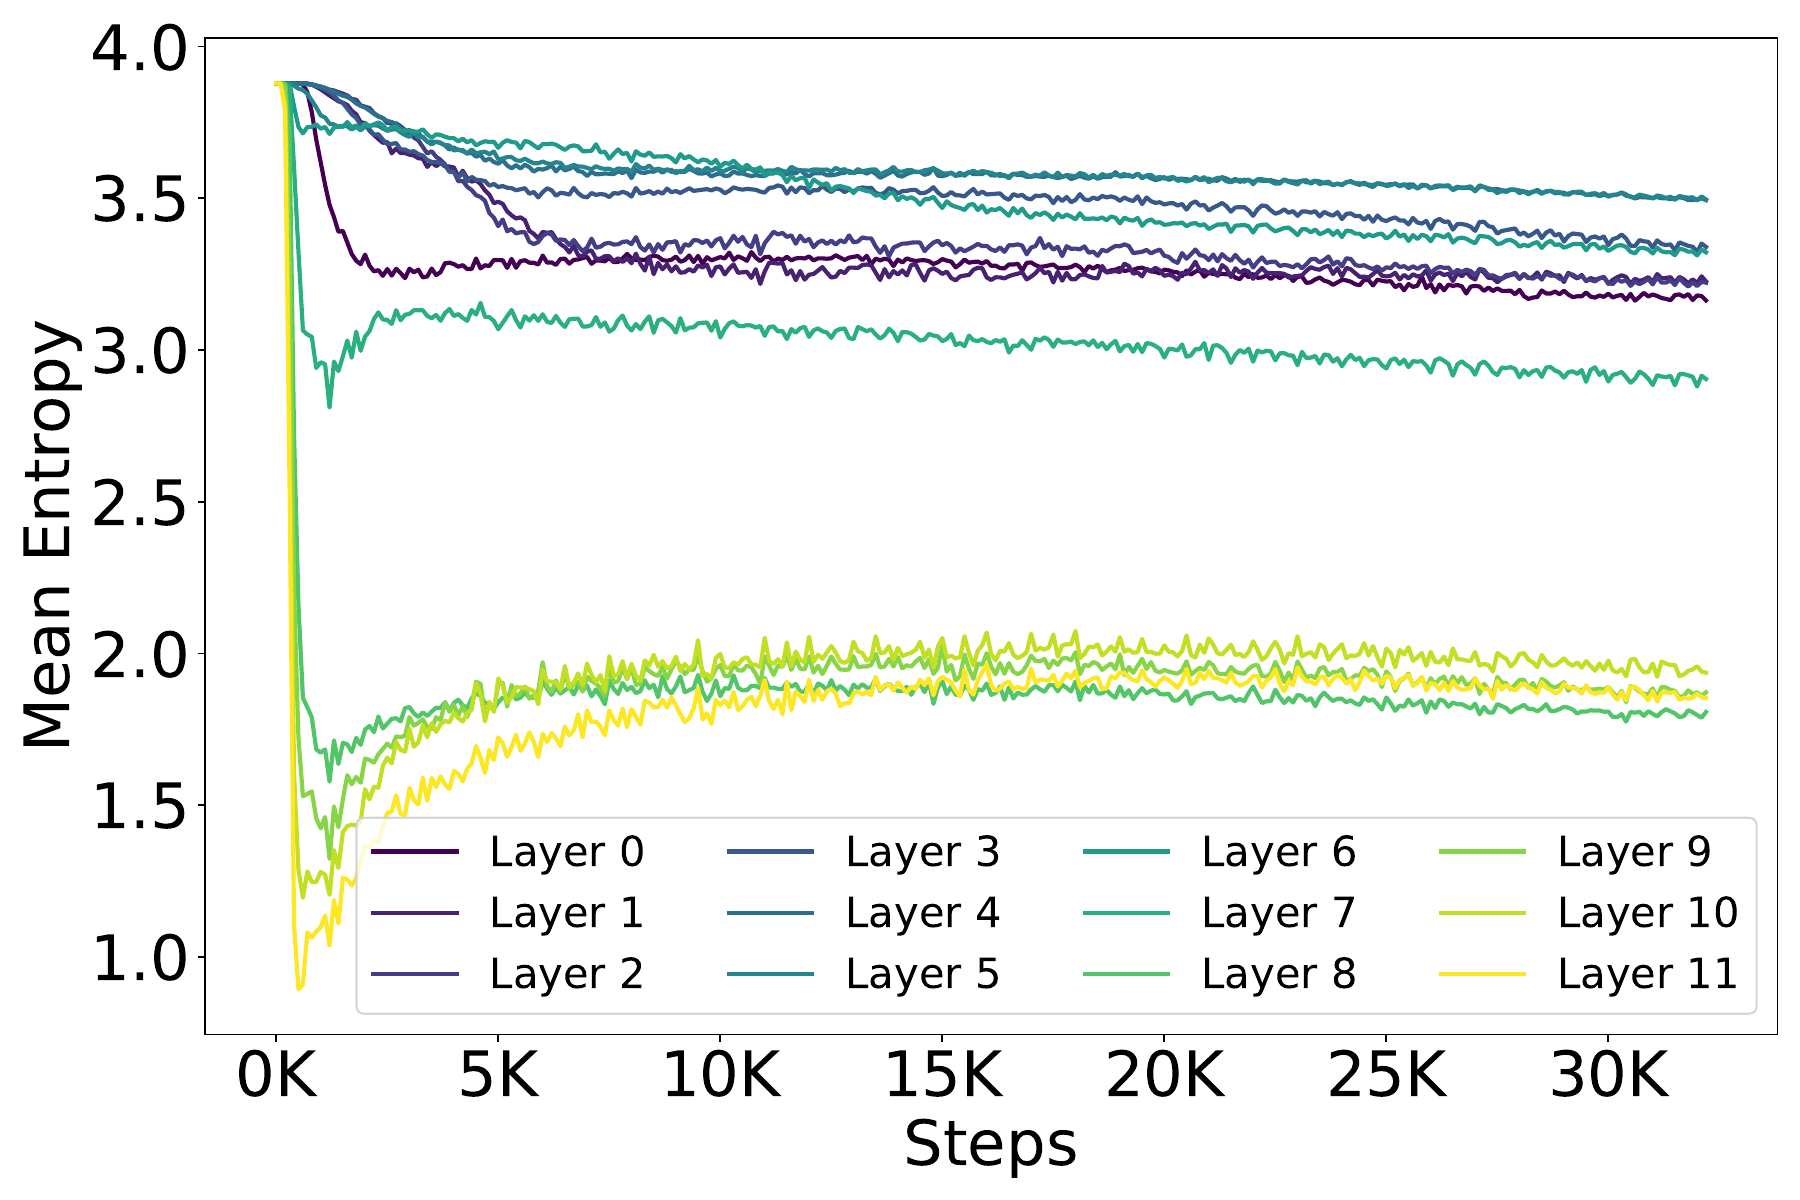}} \\
\subfloat[SM + R]{\includegraphics[width=.49\textwidth]{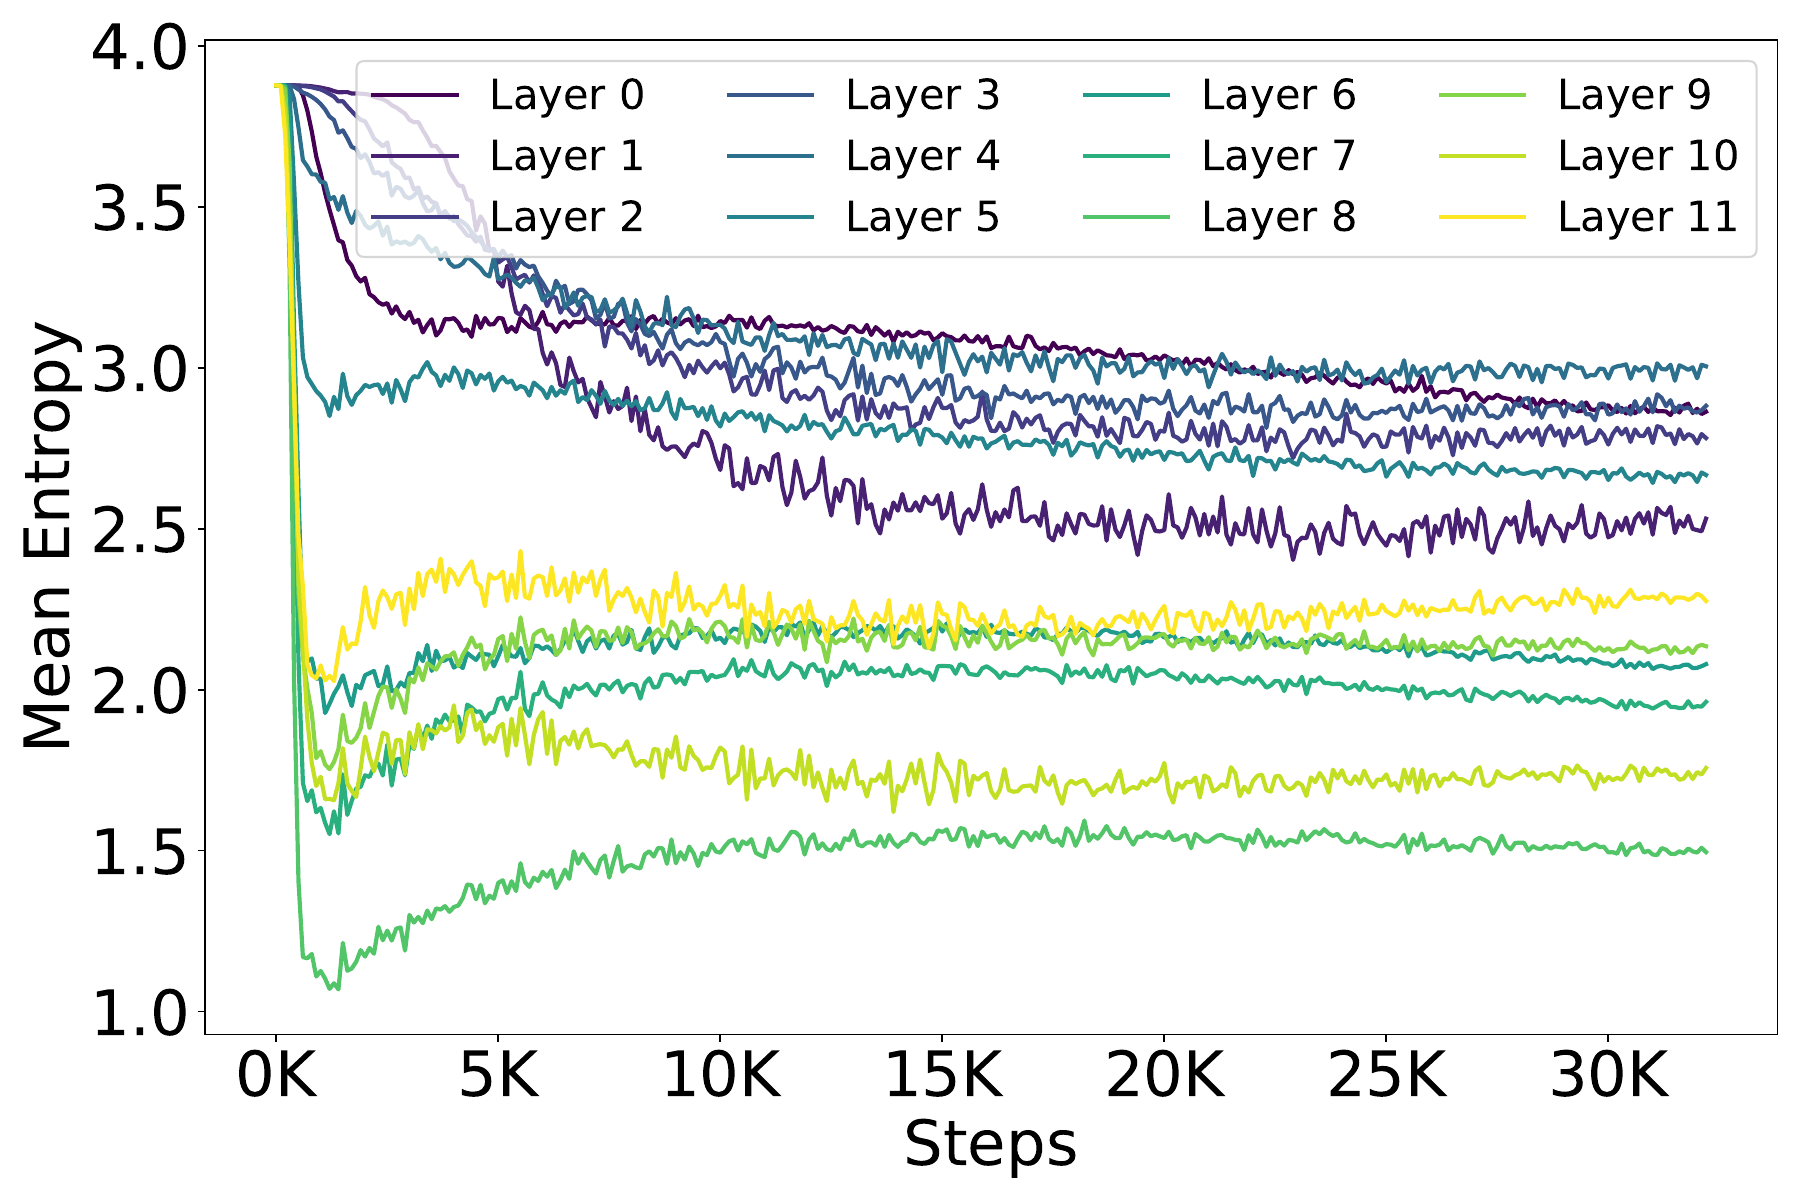}} 
\subfloat[SM ]{\includegraphics[width=.49\textwidth]{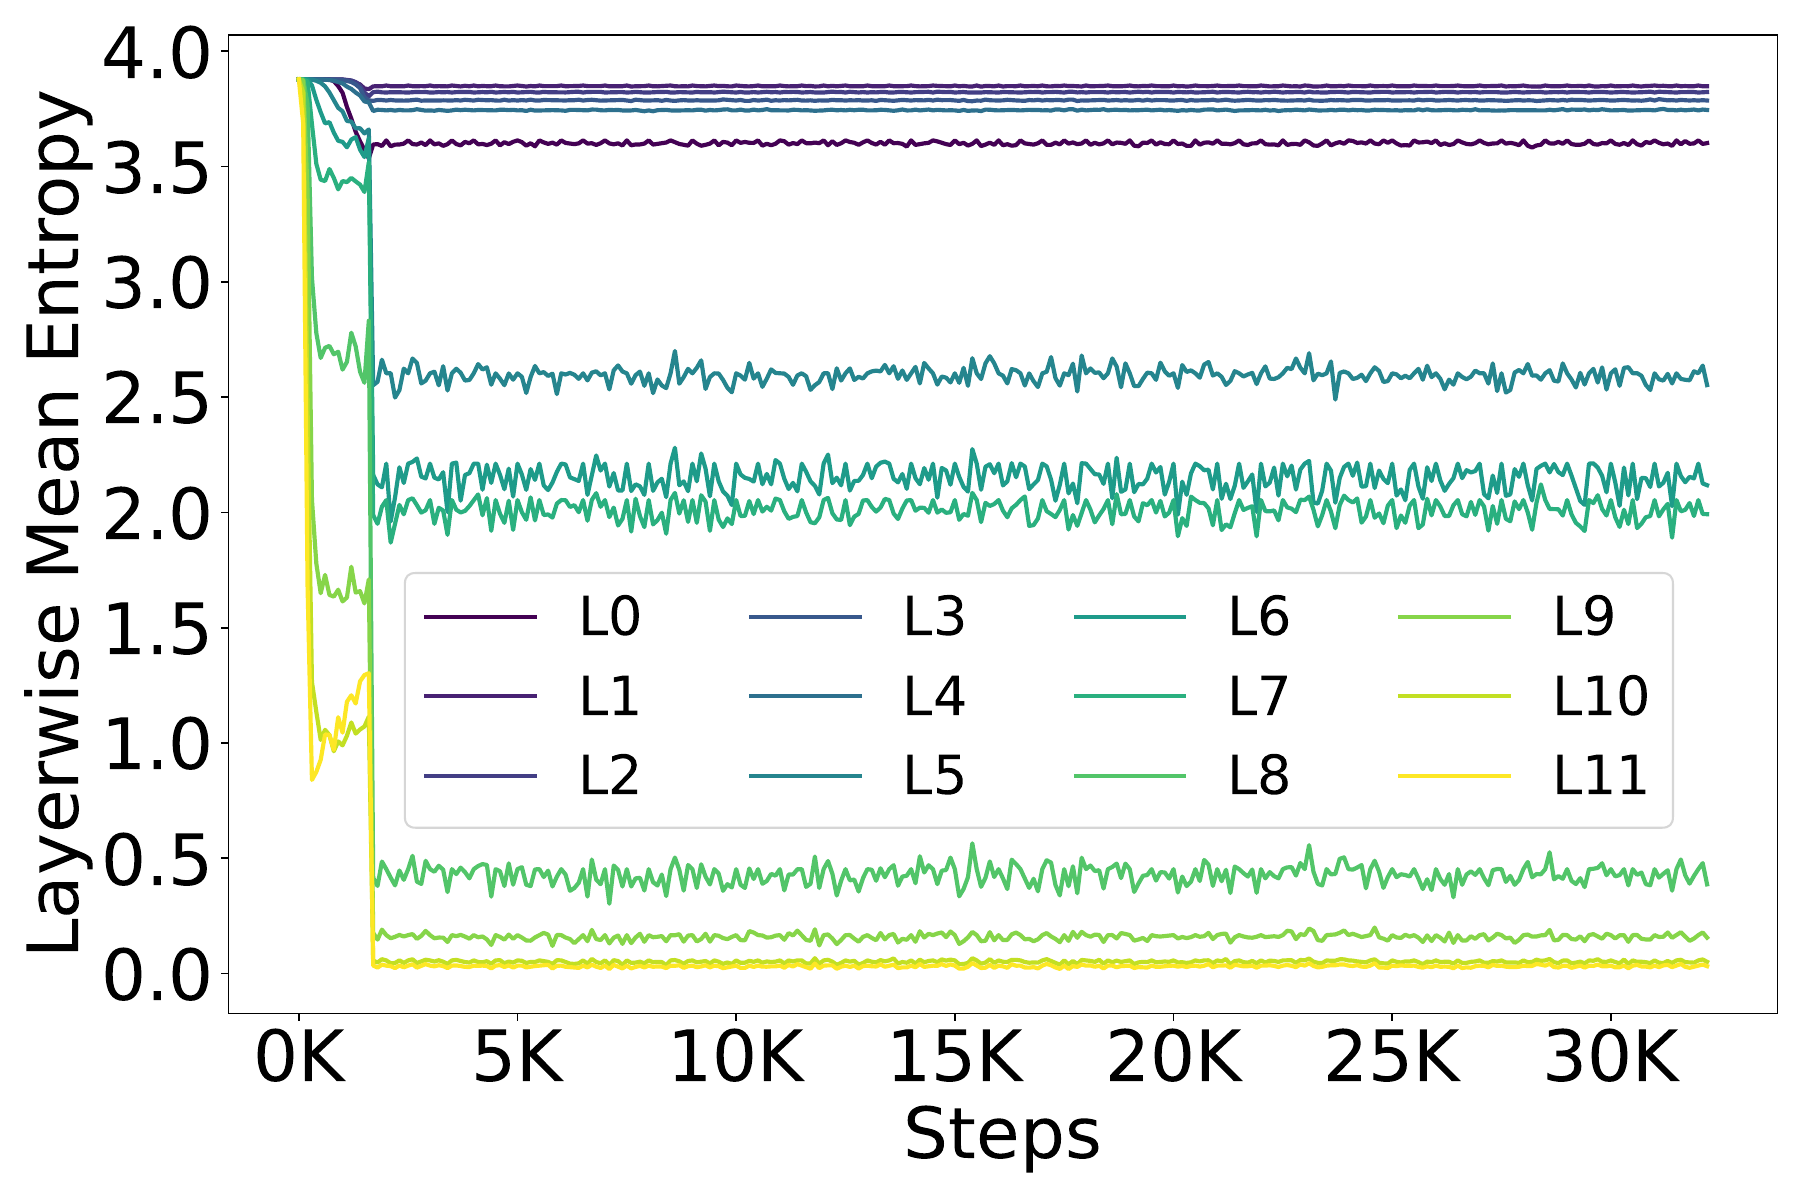}} 
\caption{Evolution of Layerwise entropy when GPT-2 ($L$=12, $H$=12, $d$=768) models with various nonlinearity configurations are trained from scratch on CodeParrot dataset. } 
\label{fig:LayerwiseEntropy}
\end{figure}
