# Supplementary material for: Entropy-Guided Attention for Private LLMs
Source: arXiv:2501.03489 source file (2025-01-08)
Supplement: Supplementary file 3 [file 22_fig_appendix_entropy_learnable_slope.tex]

\begin{figure} [htbp]
\centering
\subfloat[Layerwise learnable slope ]{\includegraphics[width=.5\textwidth]{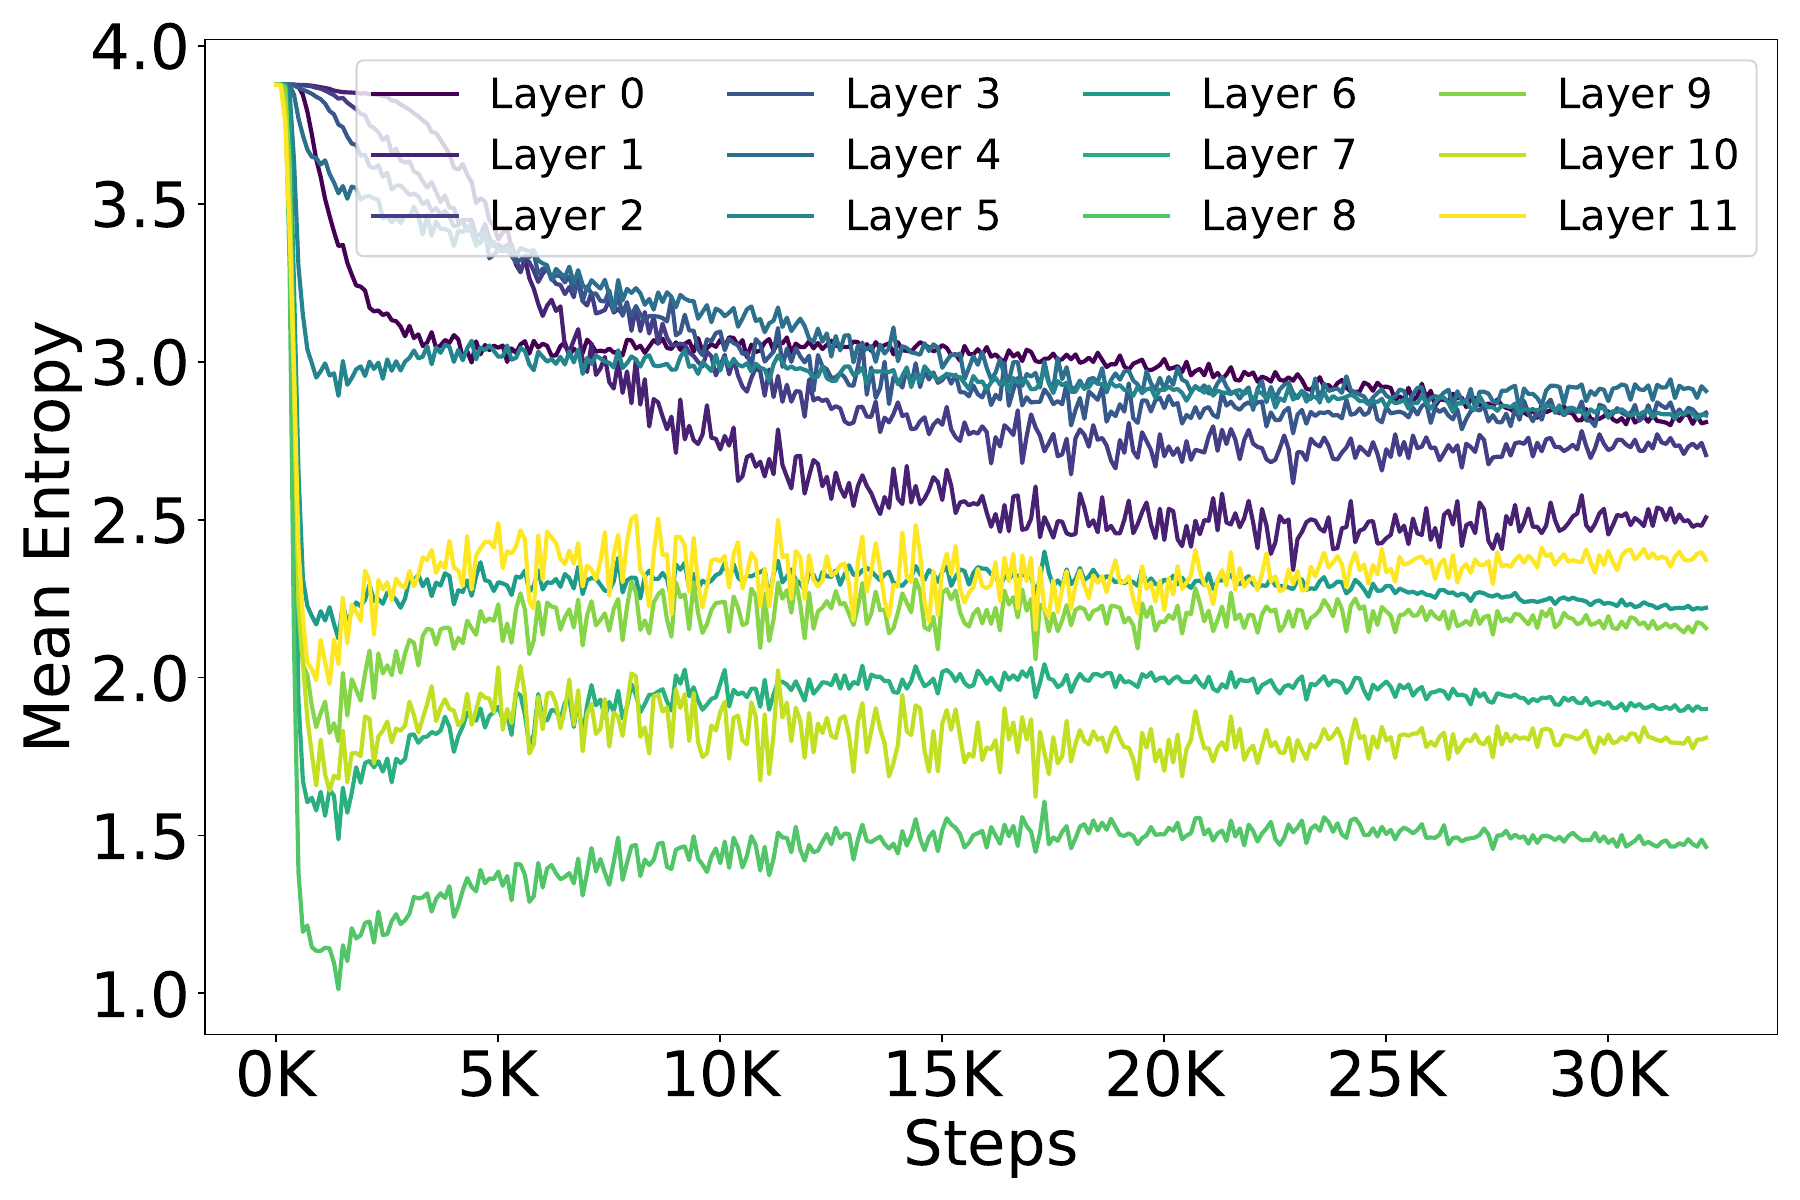}} 
\subfloat[Global slope]{\includegraphics[width=.5\textwidth]{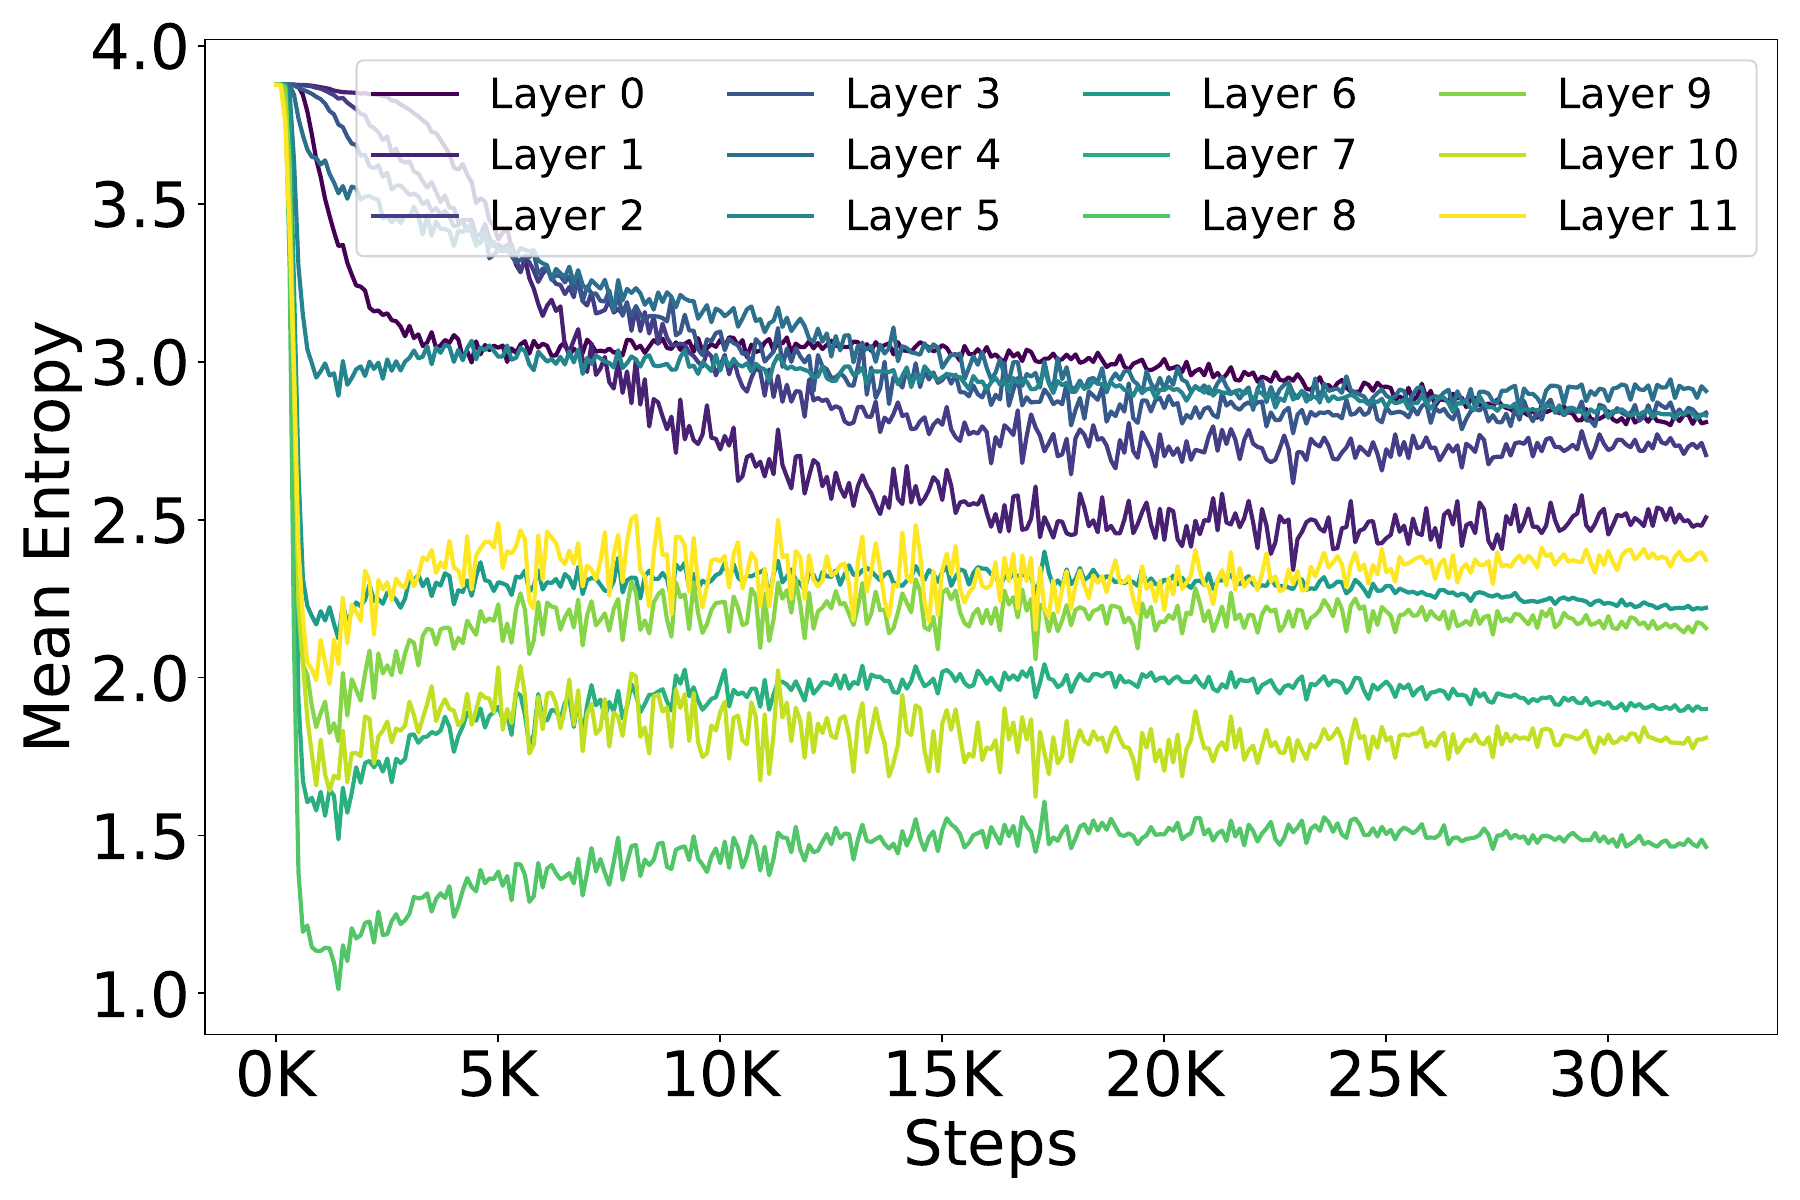}} 
\caption{Evolution of layerwise entropy in LayerNorm-free GPT-2 models ($L$ = 12, $H$ = 12, $d$ = 768) with a learnable negative slope in the leaky ReLU activation function, trained from scratch on the CodeParrot dataset} 
\label{fig:LayerwiseEntropyNegSlope}
\end{figure}
