# Supplementary material for: Entropy-Guided Attention for Private LLMs
Source: arXiv:2501.03489 source file (2025-01-08)
Supplement: Supplementary file 4 [file 23_fig_appendix_scaled_ffn_values.tex]

\begin{figure} [htbp]
\centering
\subfloat[FFN output scaling factor $\alpha$ ]{\includegraphics[width=.49\textwidth]{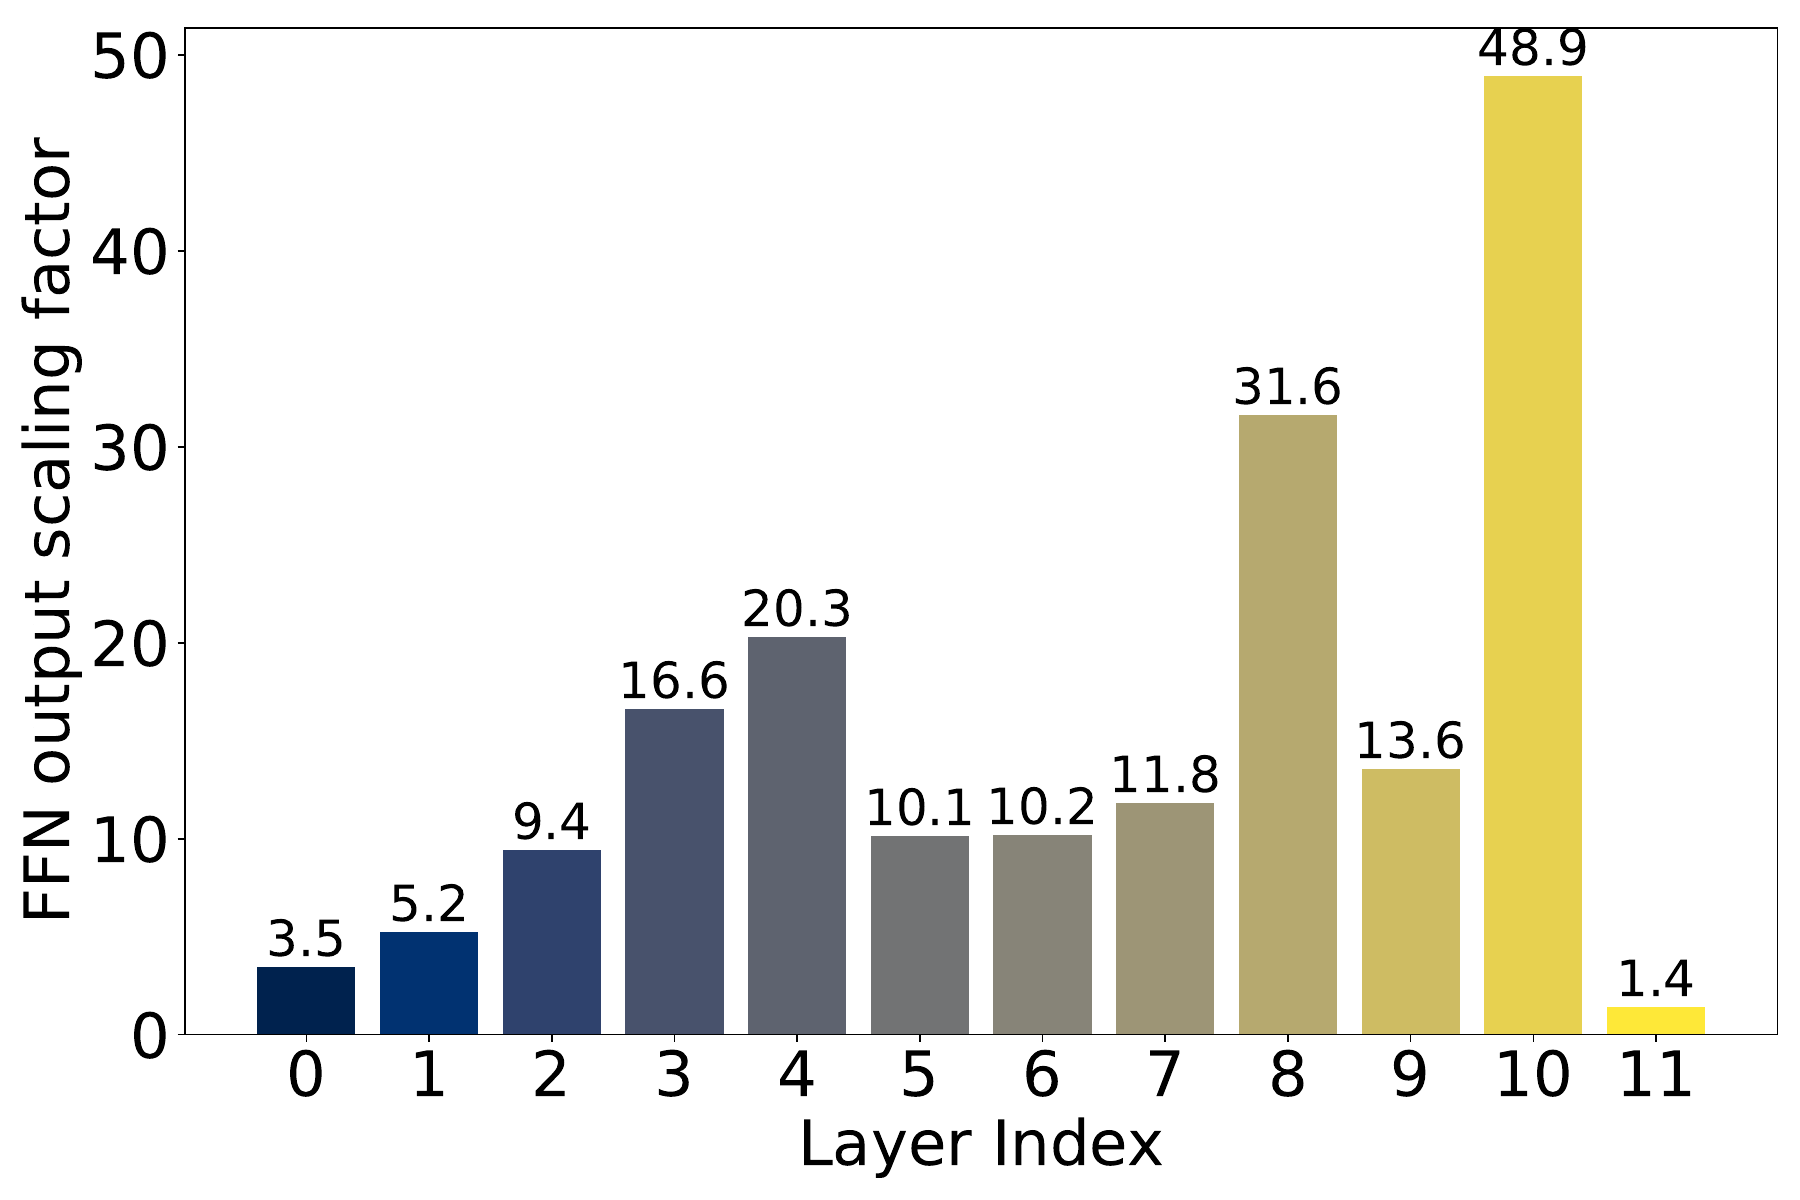}} 
\subfloat[FFN-block's residual scaling factor $\beta$]{\includegraphics[width=.49\textwidth]{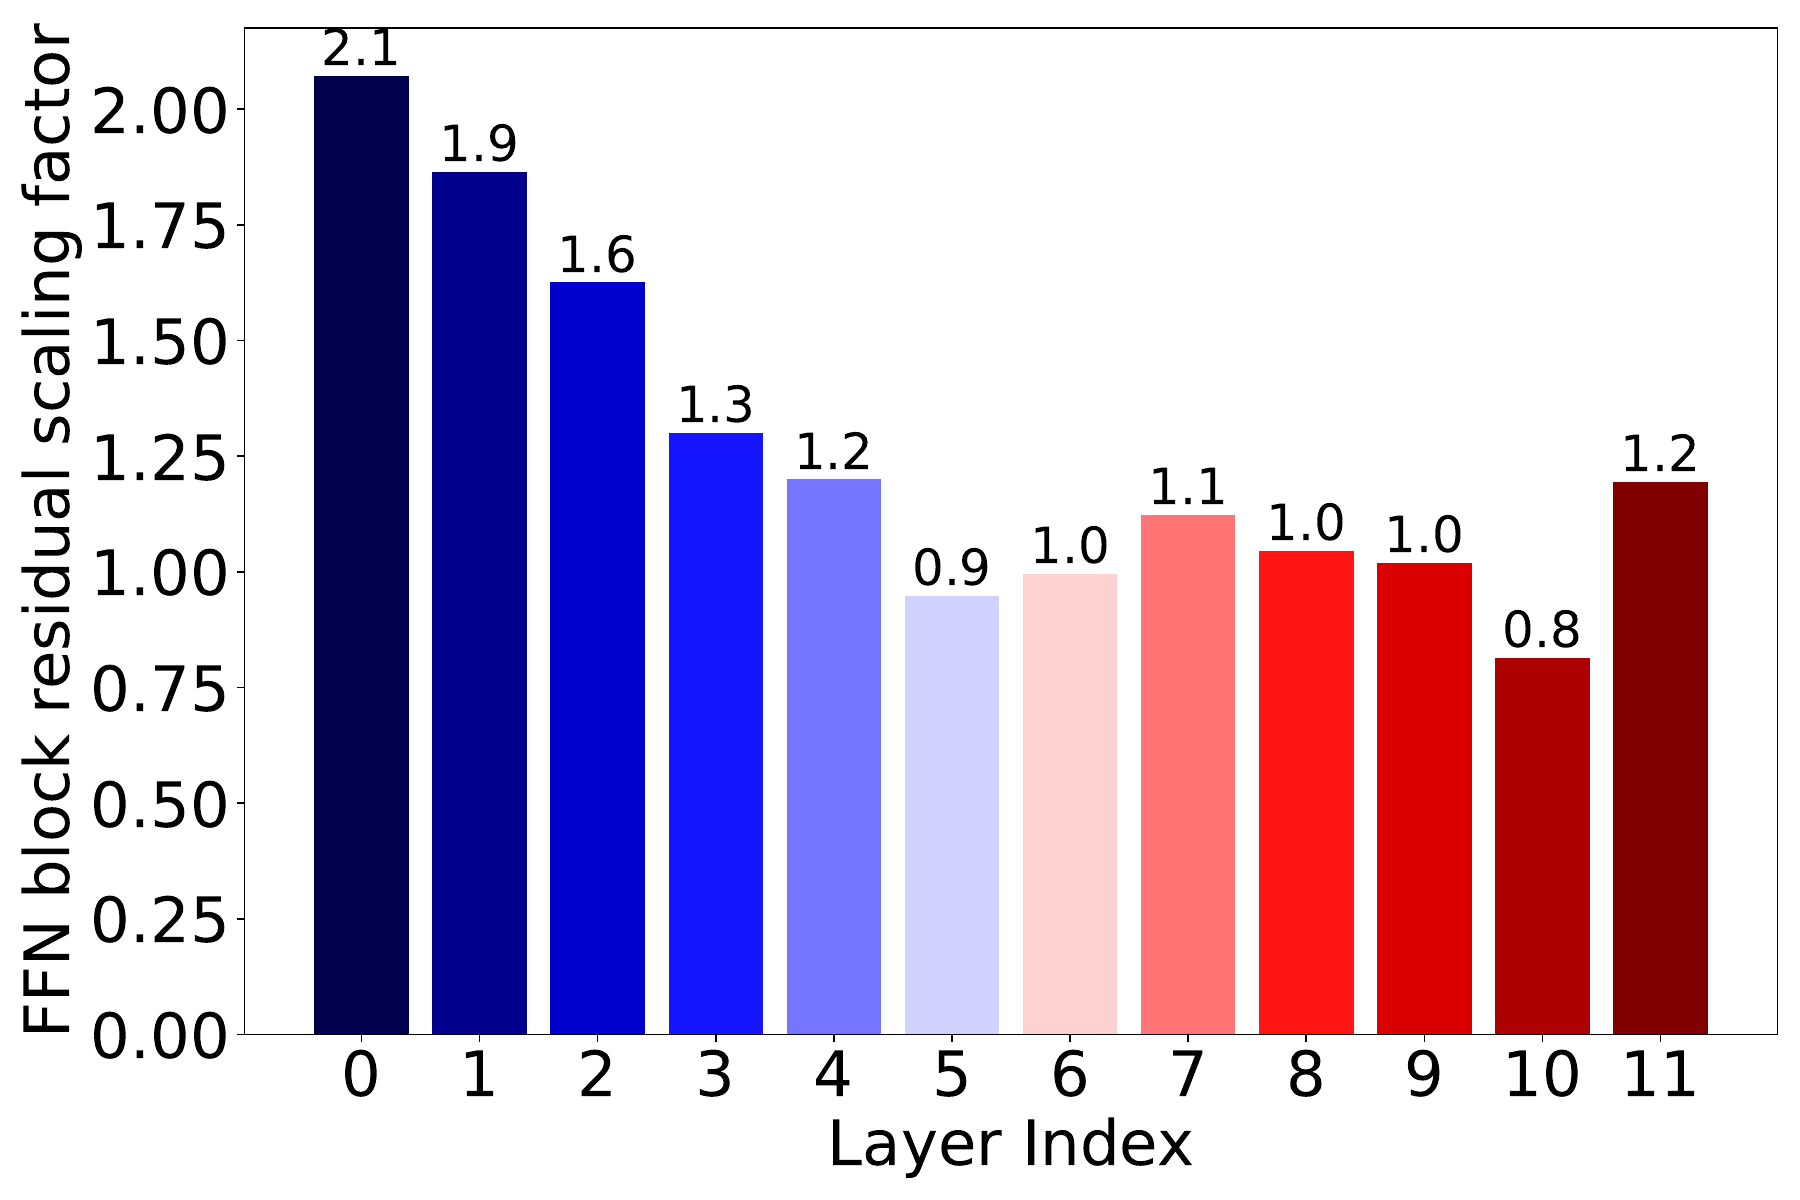}} \\ 
\caption{Learned scaling factors $\alpha$ and $\beta$ in Eq. \ref{eqn:ScaledFFN} across different layers in the Softmax-only GPT-2 model ($L$=12, $H$=12, $d$=768). The values were plotted after full model training to observe the modulation of FFN outputs and residual connections in each layer.} 
\label{fig:LearnableScalingFactor}
\end{figure}
