# Supplementary material for: Entropy-Guided Attention for Private LLMs
Source: arXiv:2501.03489 source file (2025-01-08)
Supplement: Supplementary file 5 [file 25_fig_appendix_flops_gpt.tex]

\begin{figure} [htbp]
\centering
\subfloat[GPT-2 small]{\includegraphics[width=.5\textwidth]{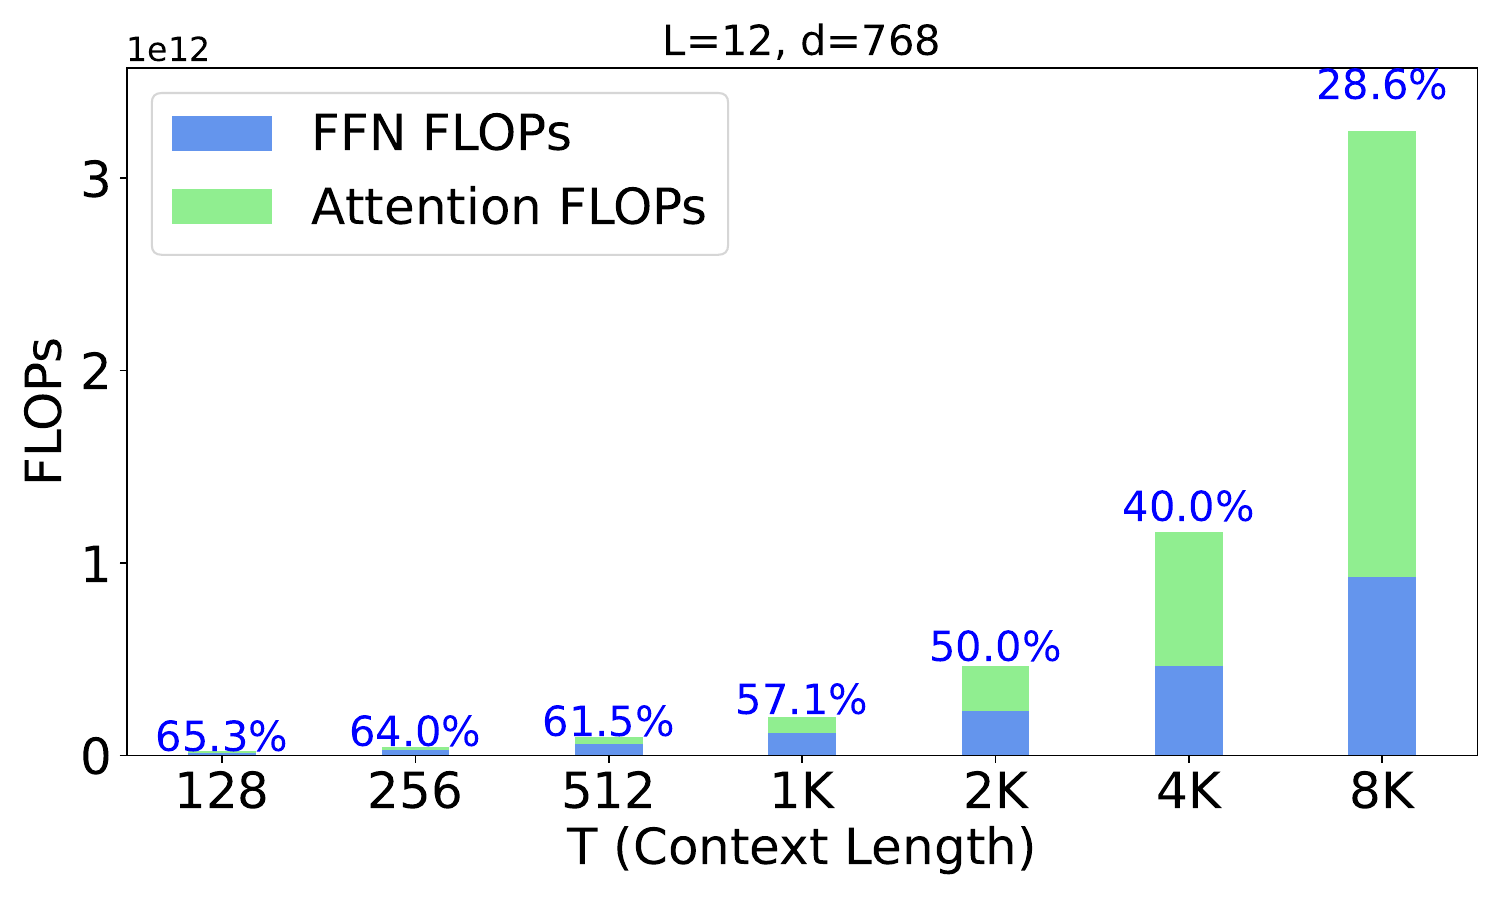}} 
\subfloat[GPT-2 medium]{\includegraphics[width=.5\textwidth]{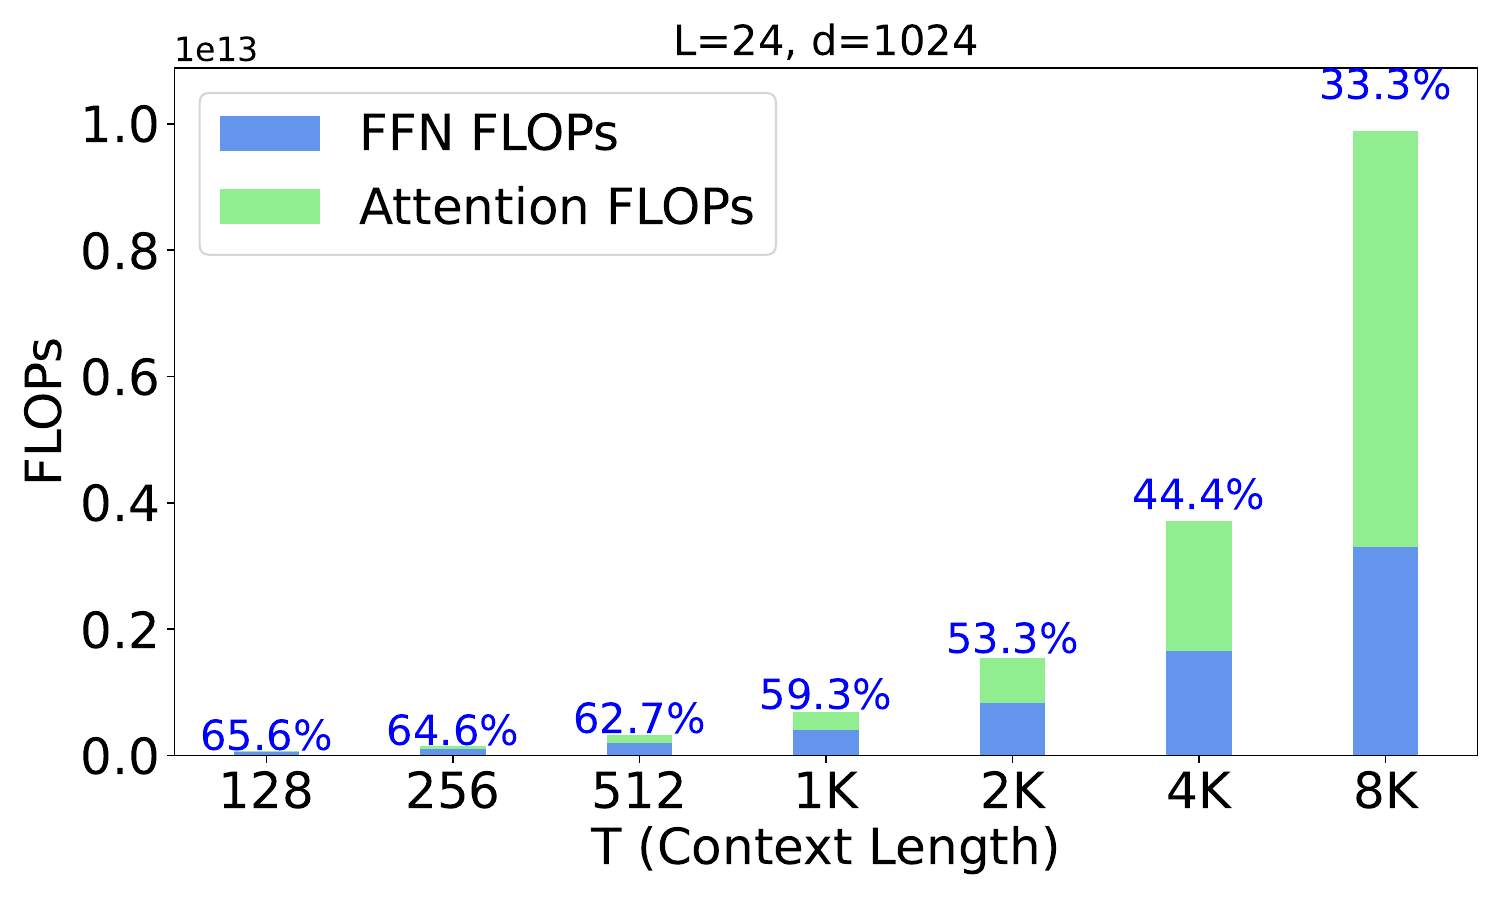}} \\ \vspace{-0.8em}
\subfloat[GPT-2 large ]{\includegraphics[width=.5\textwidth]{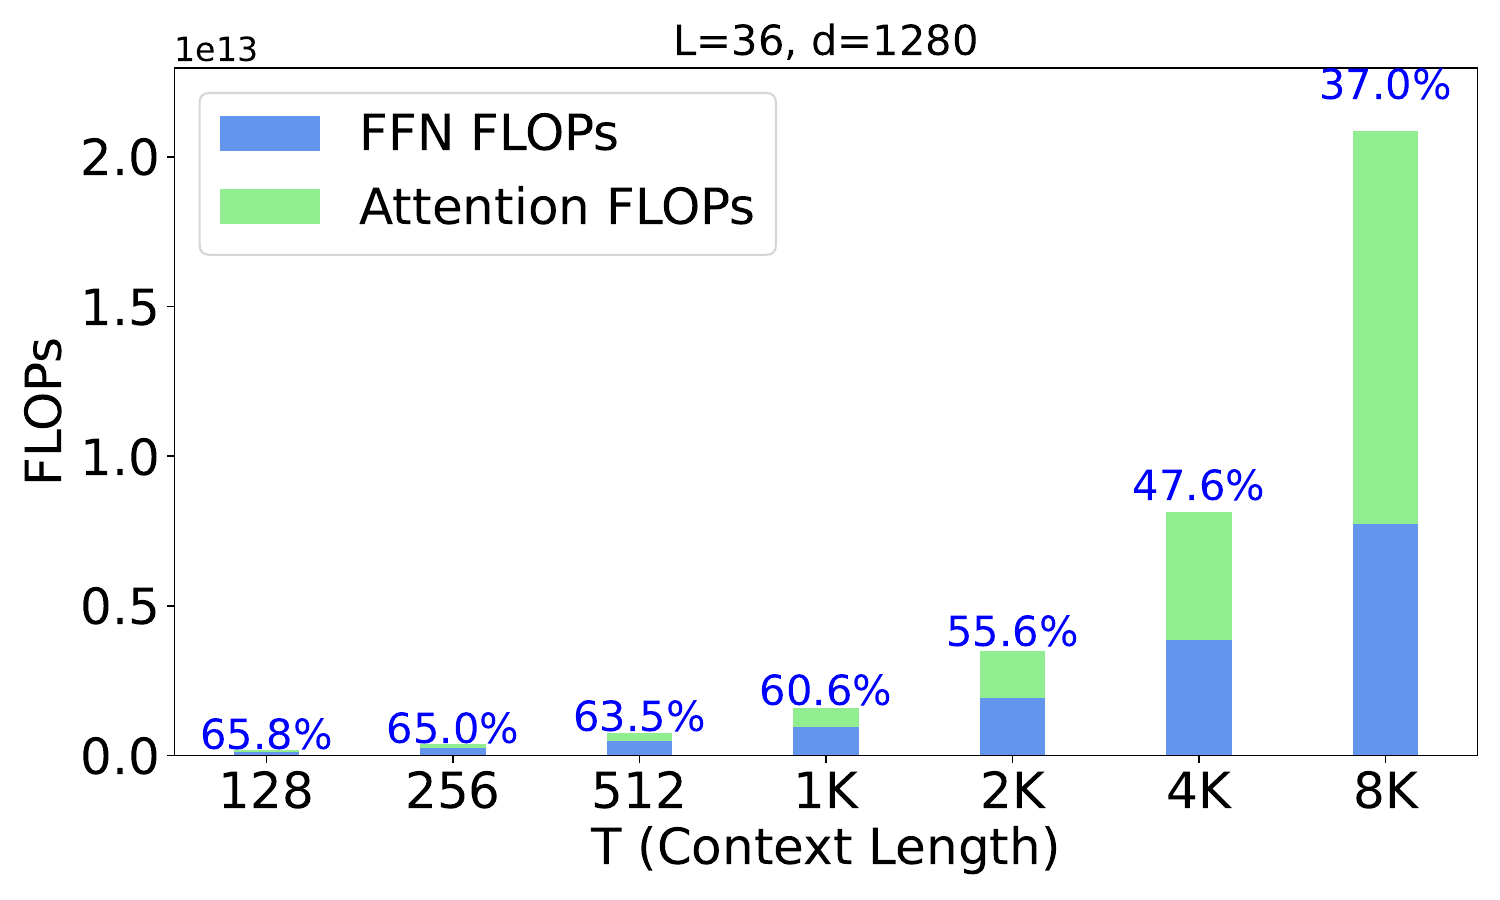}} 
\subfloat[GPT-2 XL]{\includegraphics[width=.5\textwidth]{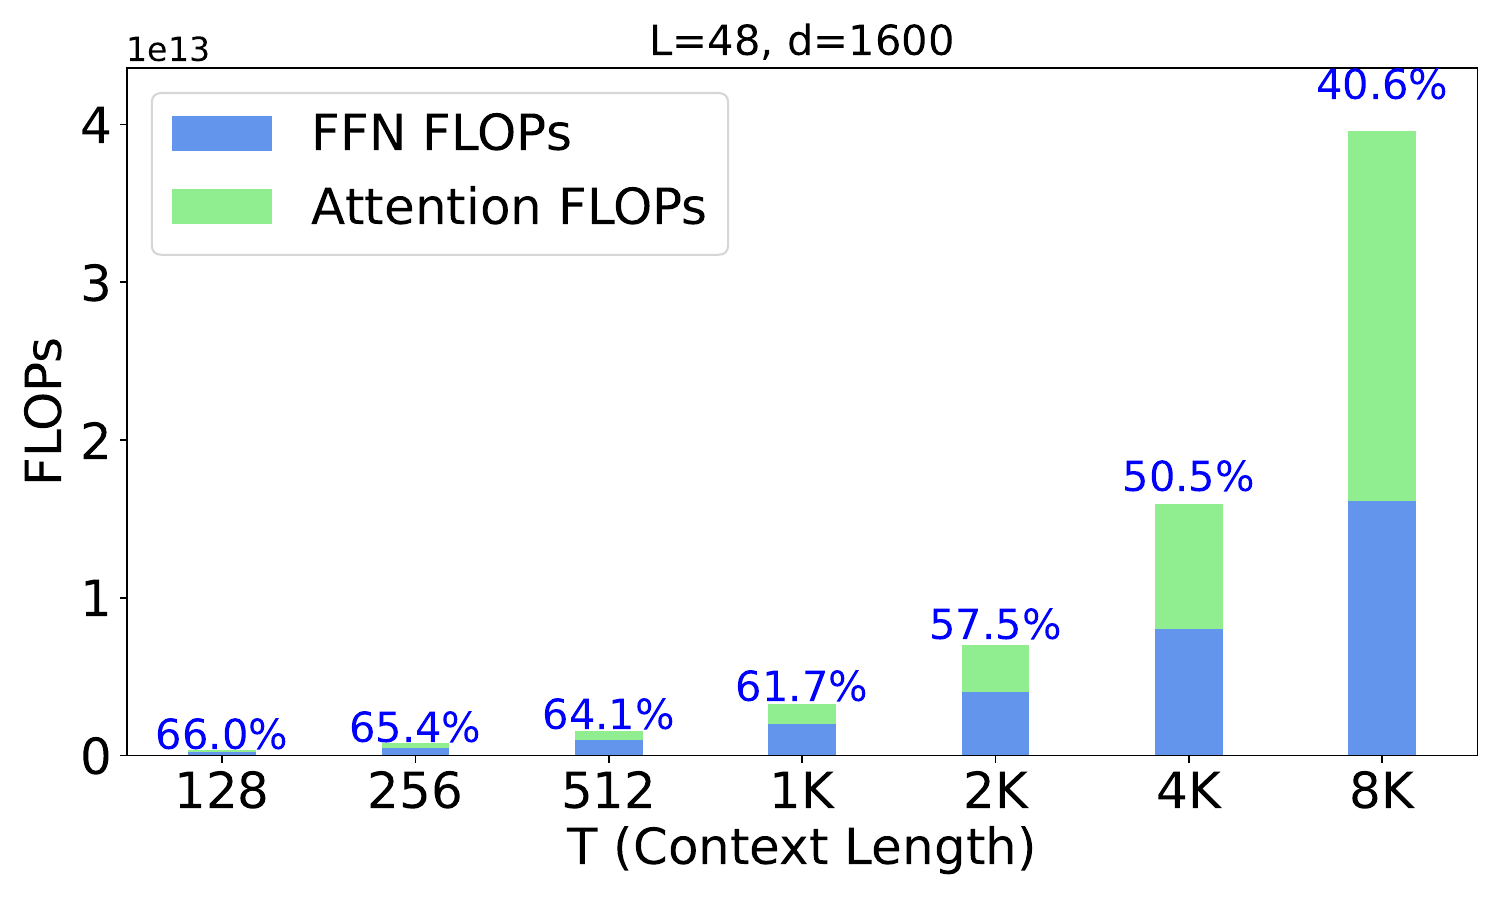}} 
\caption{FLOPs breakdown in GPT-2 models for a single forward pass: Up to a context length of 2K, FFN operations are the primary contributors to FLOPs. Beyond 8K, attention operations start to dominate (Percentage on top of each bar represents the proportion of FFN FLOPs)} 
\label{fig:FlopsGPT}
\end{figure}
