# Supplementary material for: Entropy-Guided Attention for Private LLMs
Source: arXiv:2501.03489 source file (2025-01-08)
Supplement: Supplementary file 6 [file 26_fig_appendix_flops_pythia.tex]

\begin{figure} [htbp]
\centering
\subfloat[Pythia-70M]{\includegraphics[width=.5\textwidth]{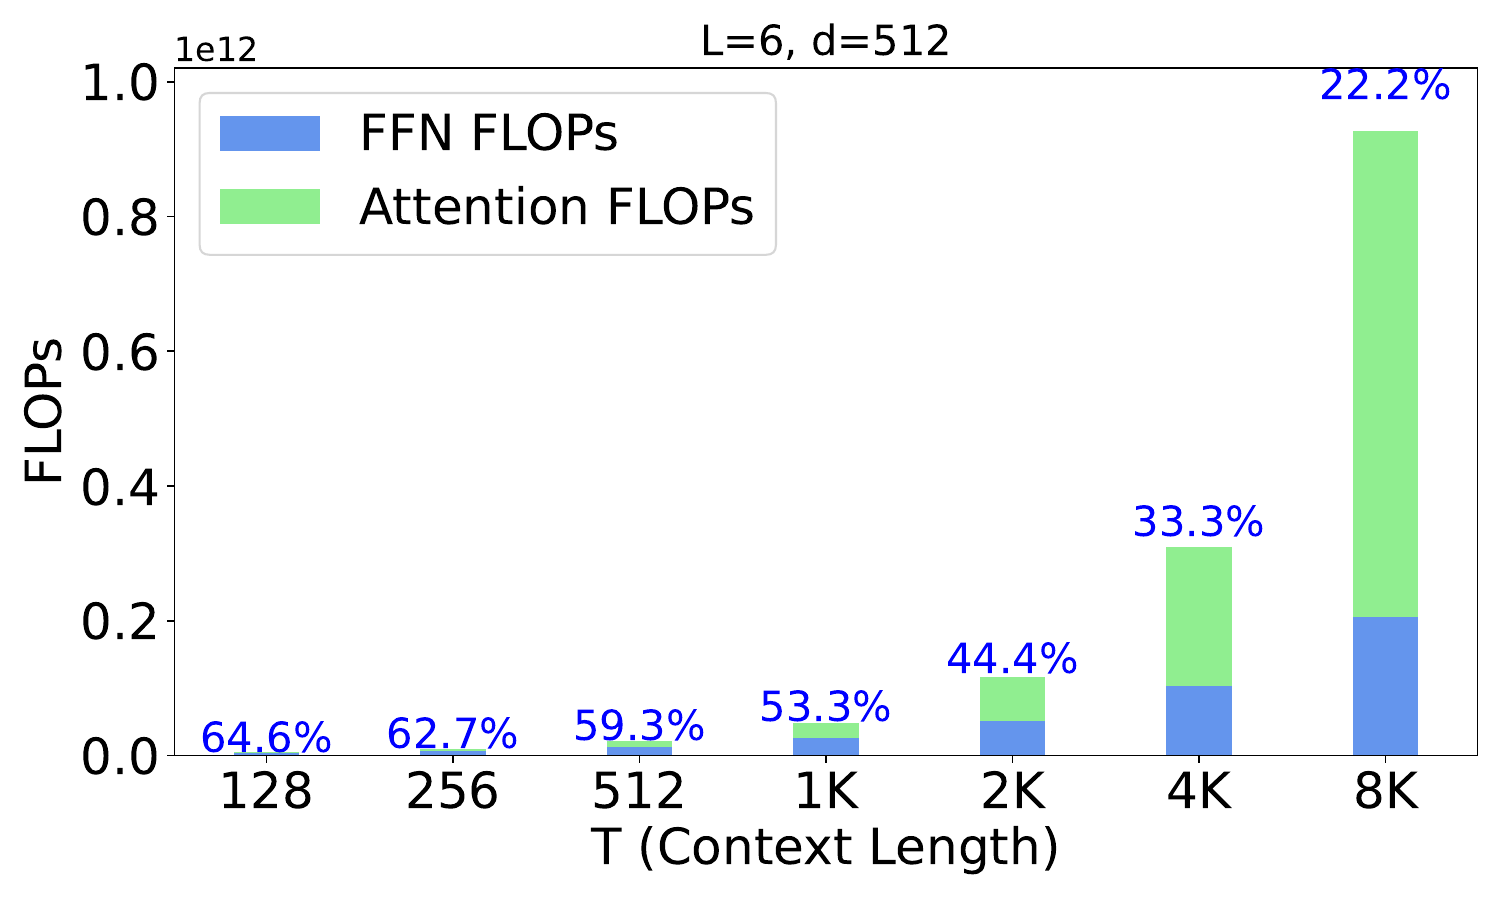}} 
\subfloat[Pythia-160M]{\includegraphics[width=.5\textwidth]{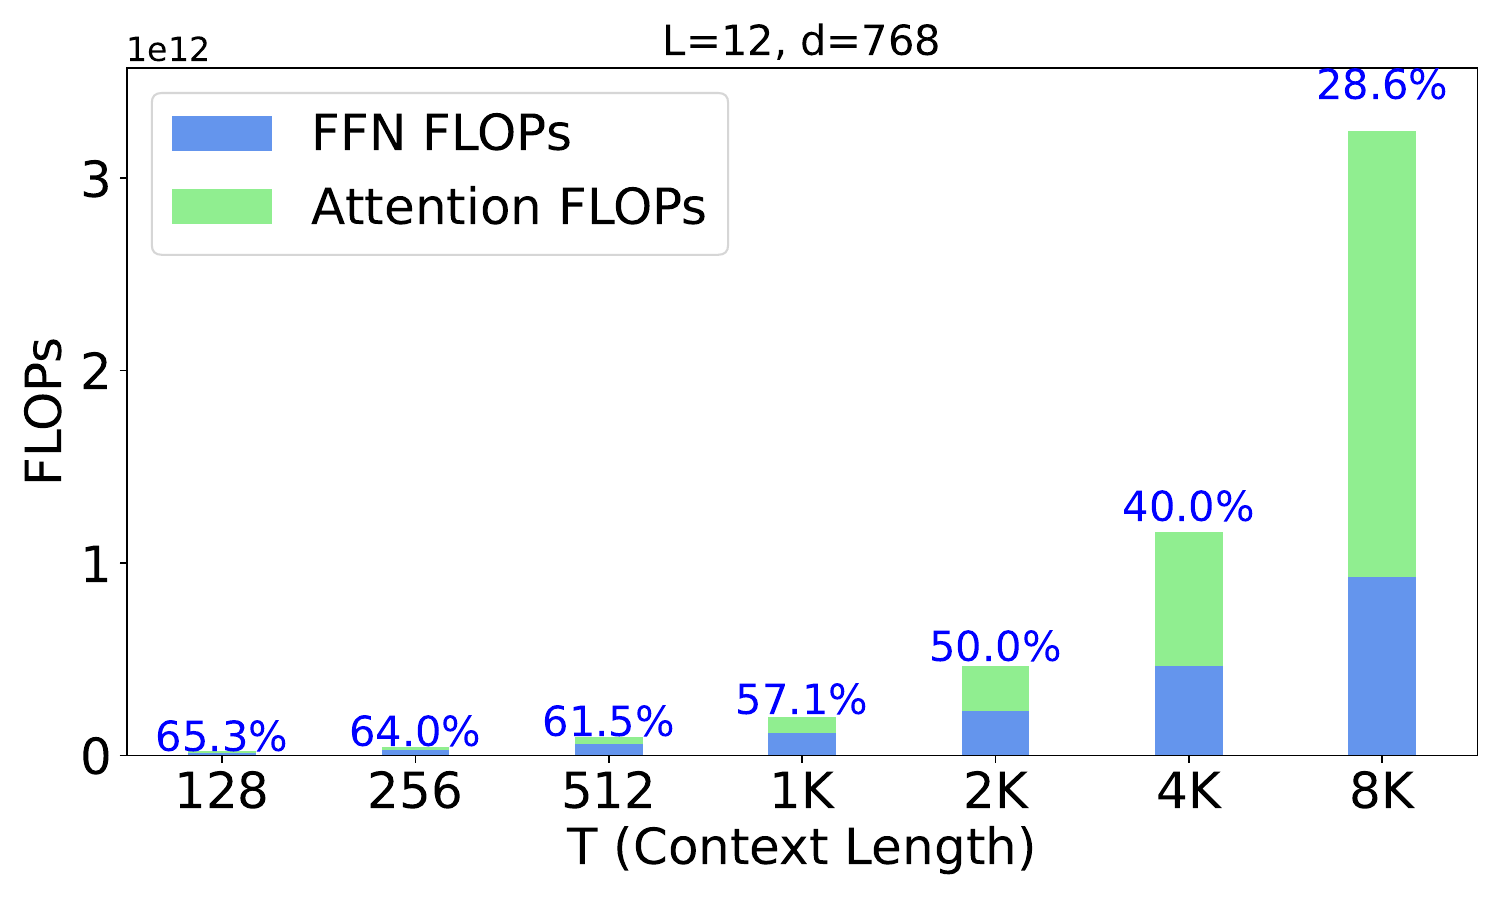}} \\  \vspace{-0.8em}
\subfloat[Pythia-410M ]{\includegraphics[width=.5\textwidth]{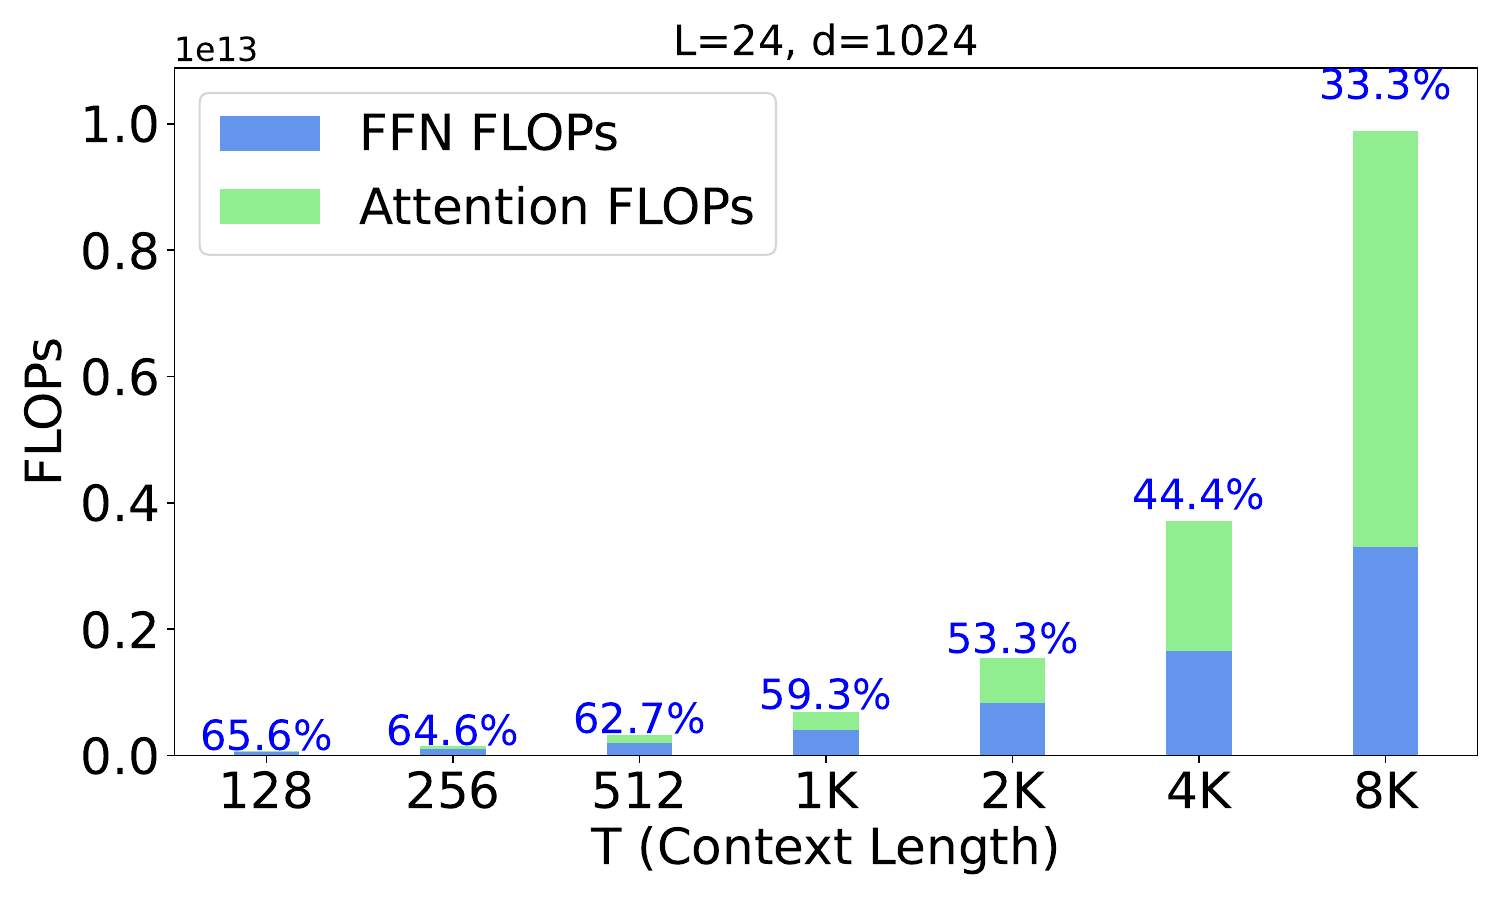}} 
\subfloat[Pythia-1B]{\includegraphics[width=.5\textwidth]{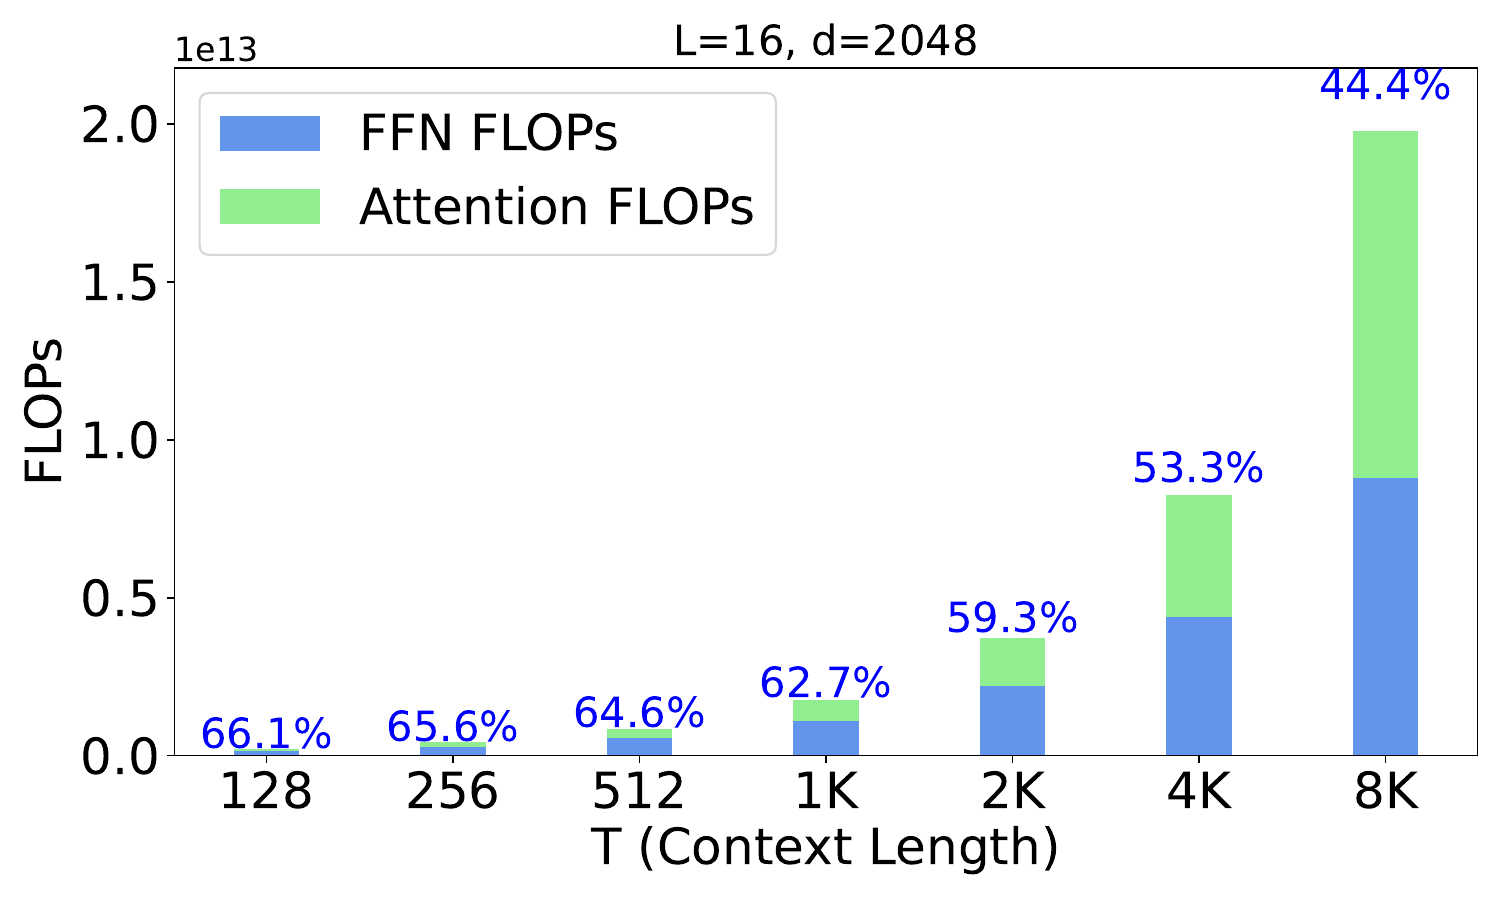}}  \\ \vspace{-0.8em}
\subfloat[Pythia-1.4B]{\includegraphics[width=.5\textwidth]{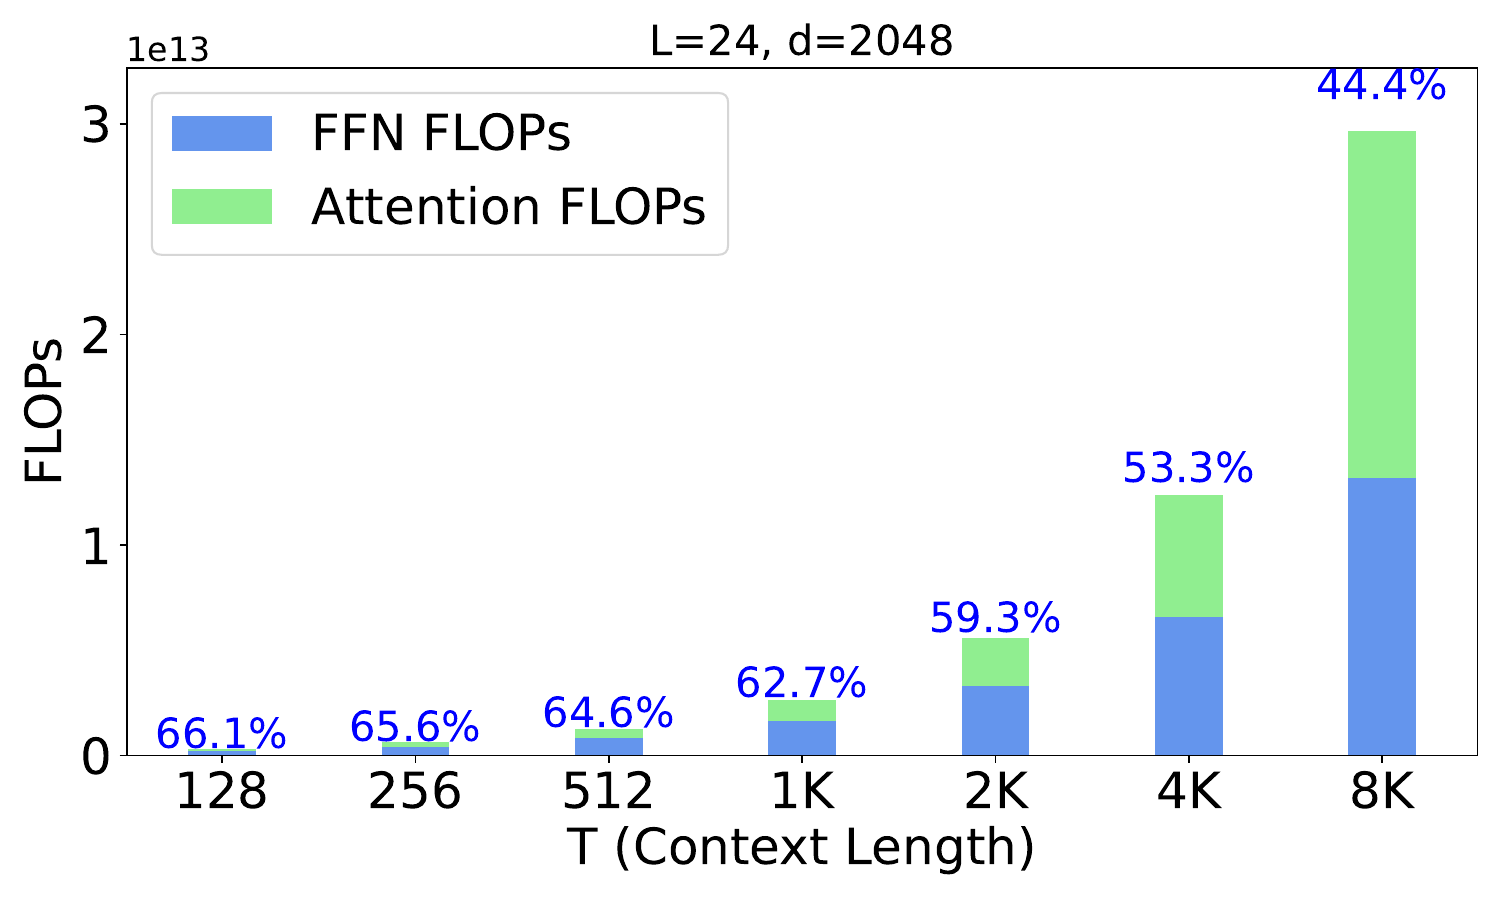}} 
\subfloat[Pythia-2.8B]{\includegraphics[width=.5\textwidth]{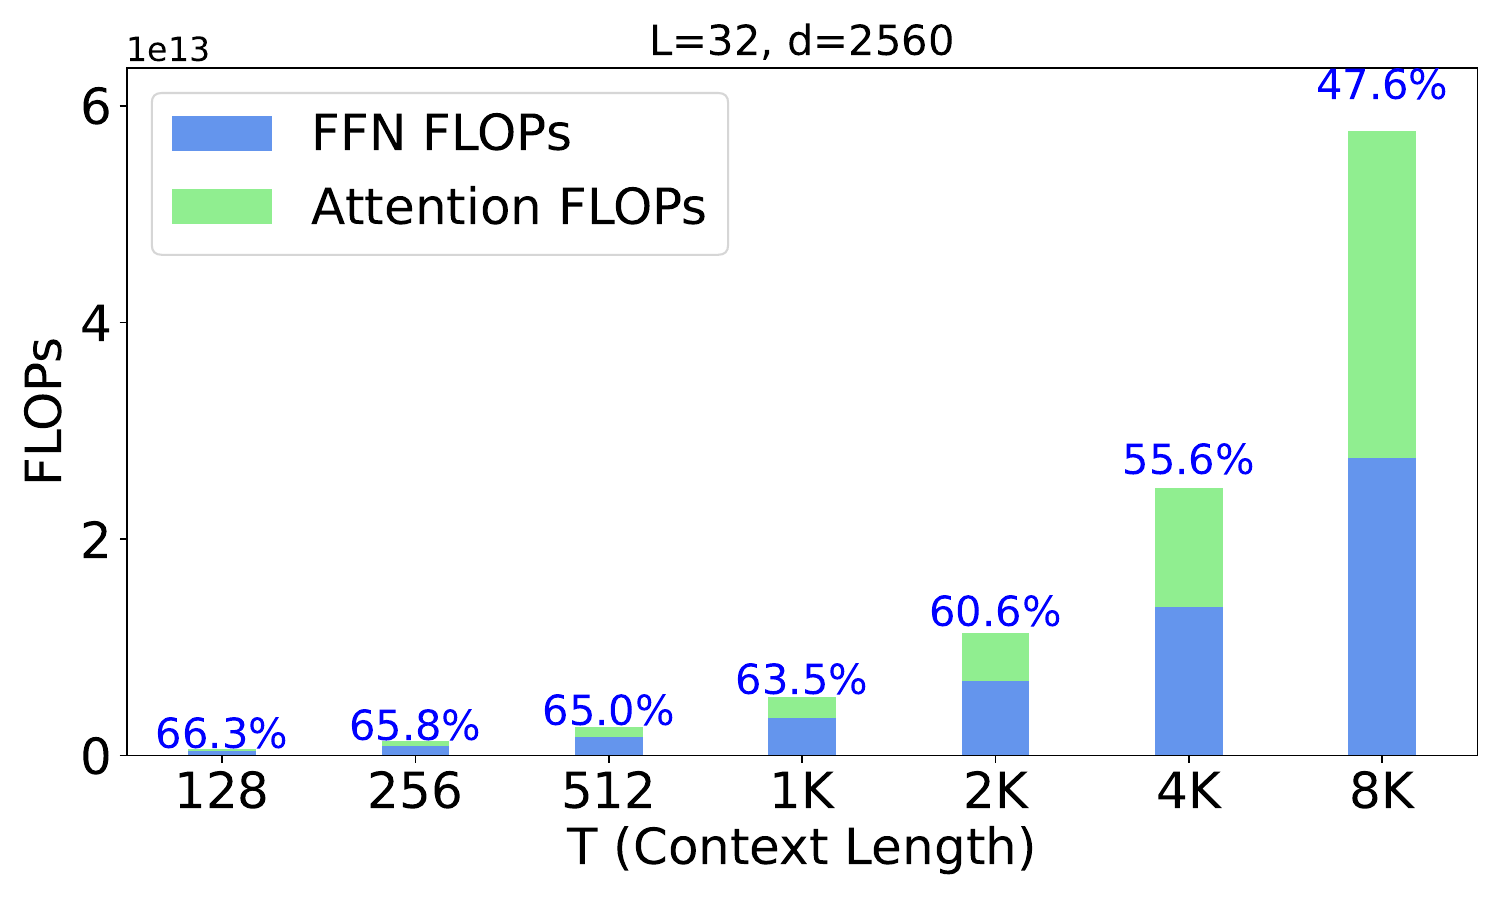}} \\ \vspace{-0.8em}
\subfloat[Pythia-6.9B]{\includegraphics[width=.5\textwidth]{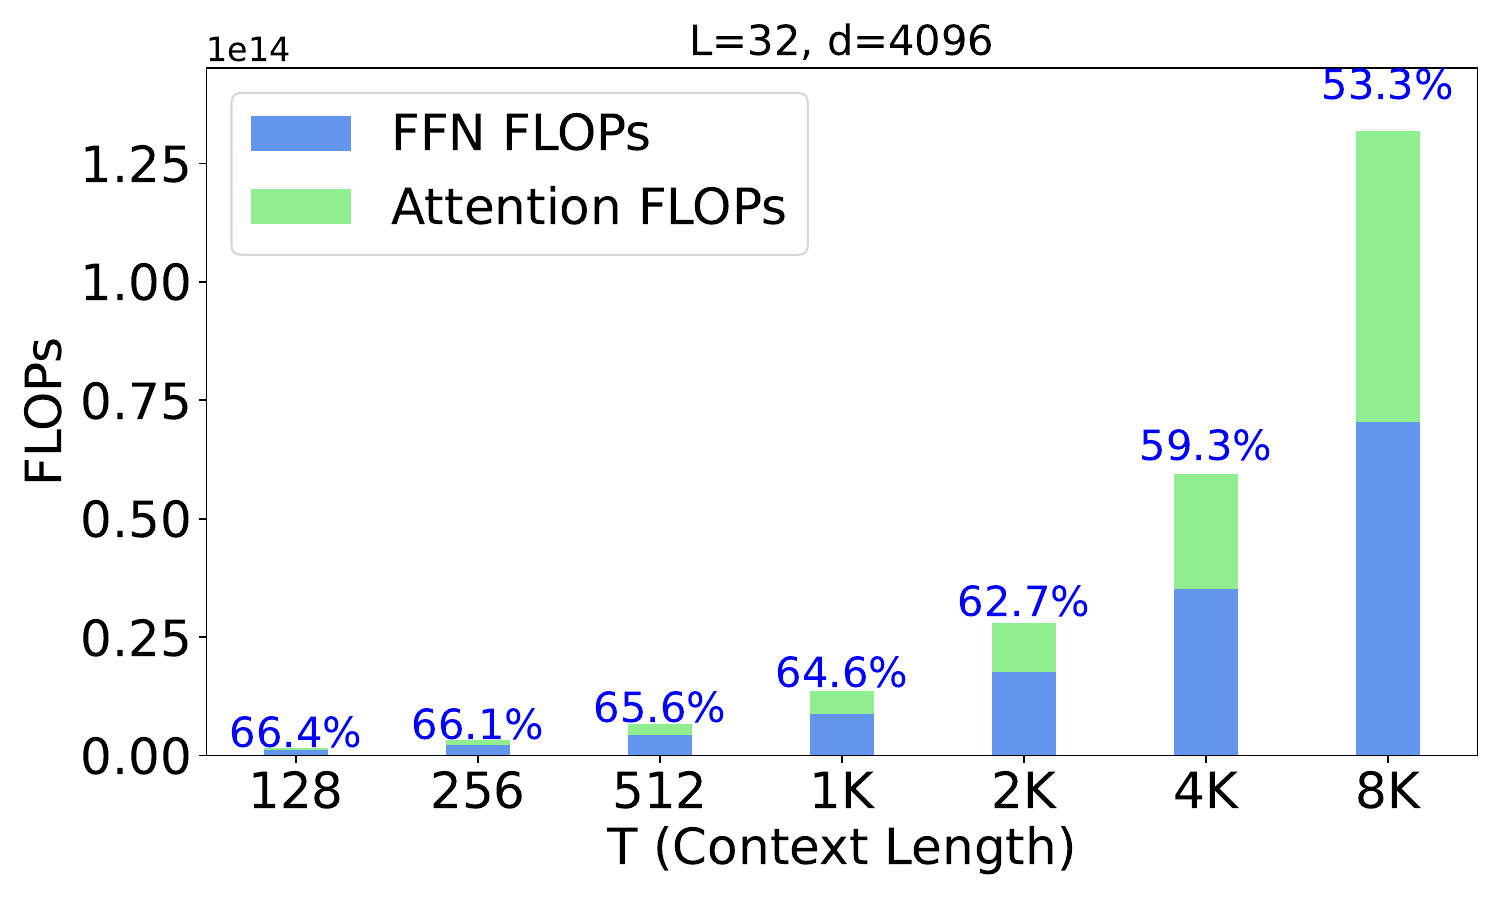}} 
\subfloat[Pythia-12B]{\includegraphics[width=.5\textwidth]{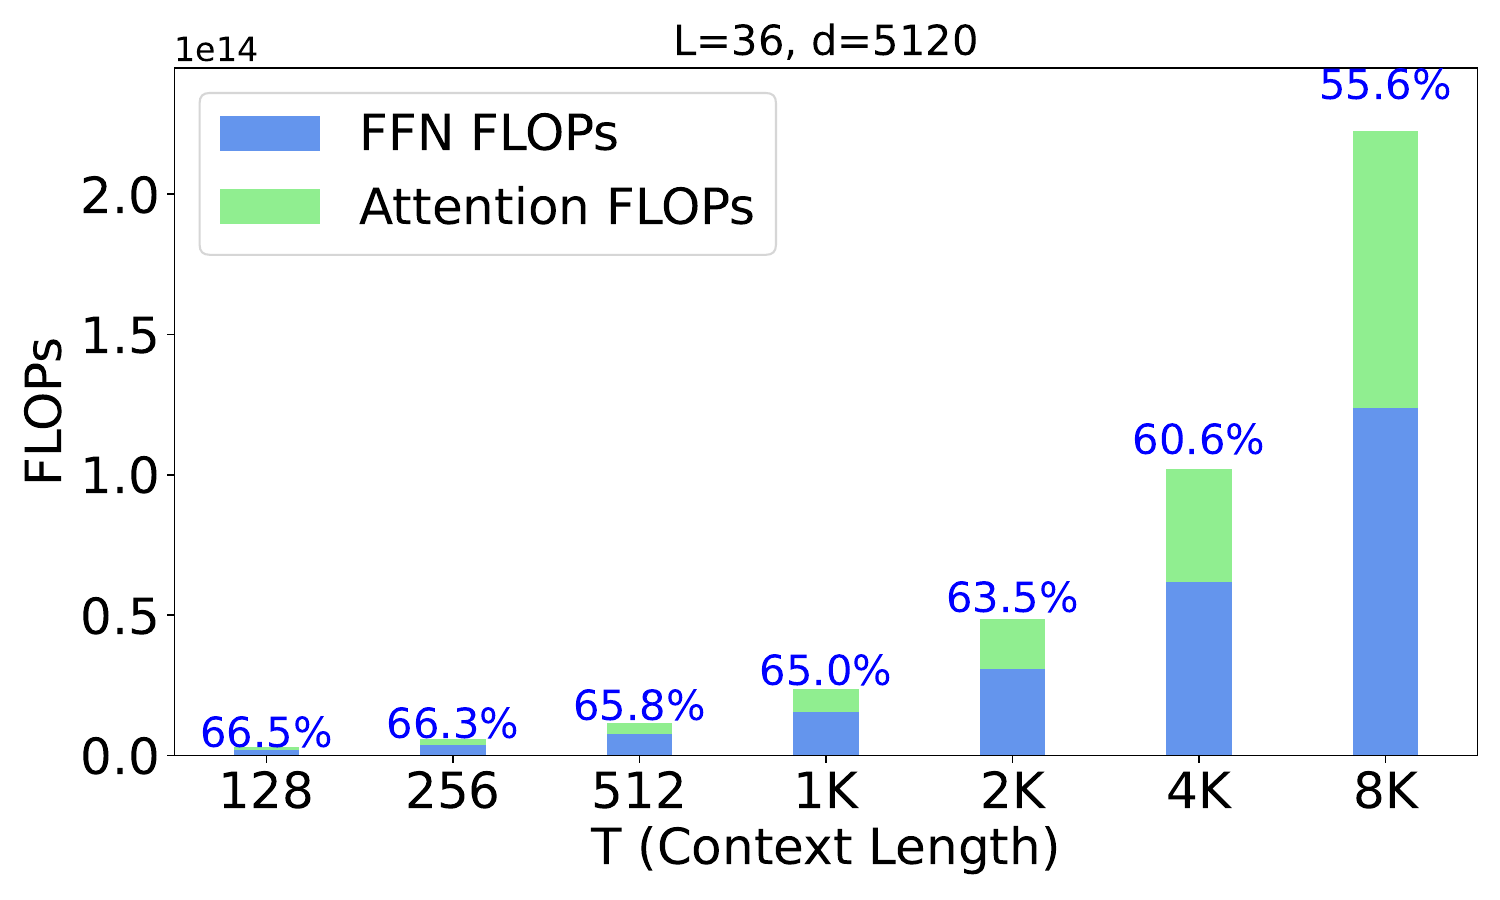}} 
\caption{FLOPs breakdown in Pythia models for a single forward pass: Similar to GPT-2 models (see Figure \ref{fig:FlopsGPT}), FLOPs are dominated by FFN operations up to a context length of 4K, except for smaller models where FFN operations dominate up to 2K (Percentage on top of each bar represents the proportion of FFN FLOPs).} 
\label{fig:FlopsPythia}
\end{figure}
