# Supplementary material for: Entropy-Guided Attention for Private LLMs
Source: arXiv:2501.03489 source file (2025-01-08)
Supplement: Supplementary file 7 [file 27_fig_appendix_pythia_70M.tex]

\begin{figure} [htbp]
\centering
\includegraphics[width=.99\textwidth]{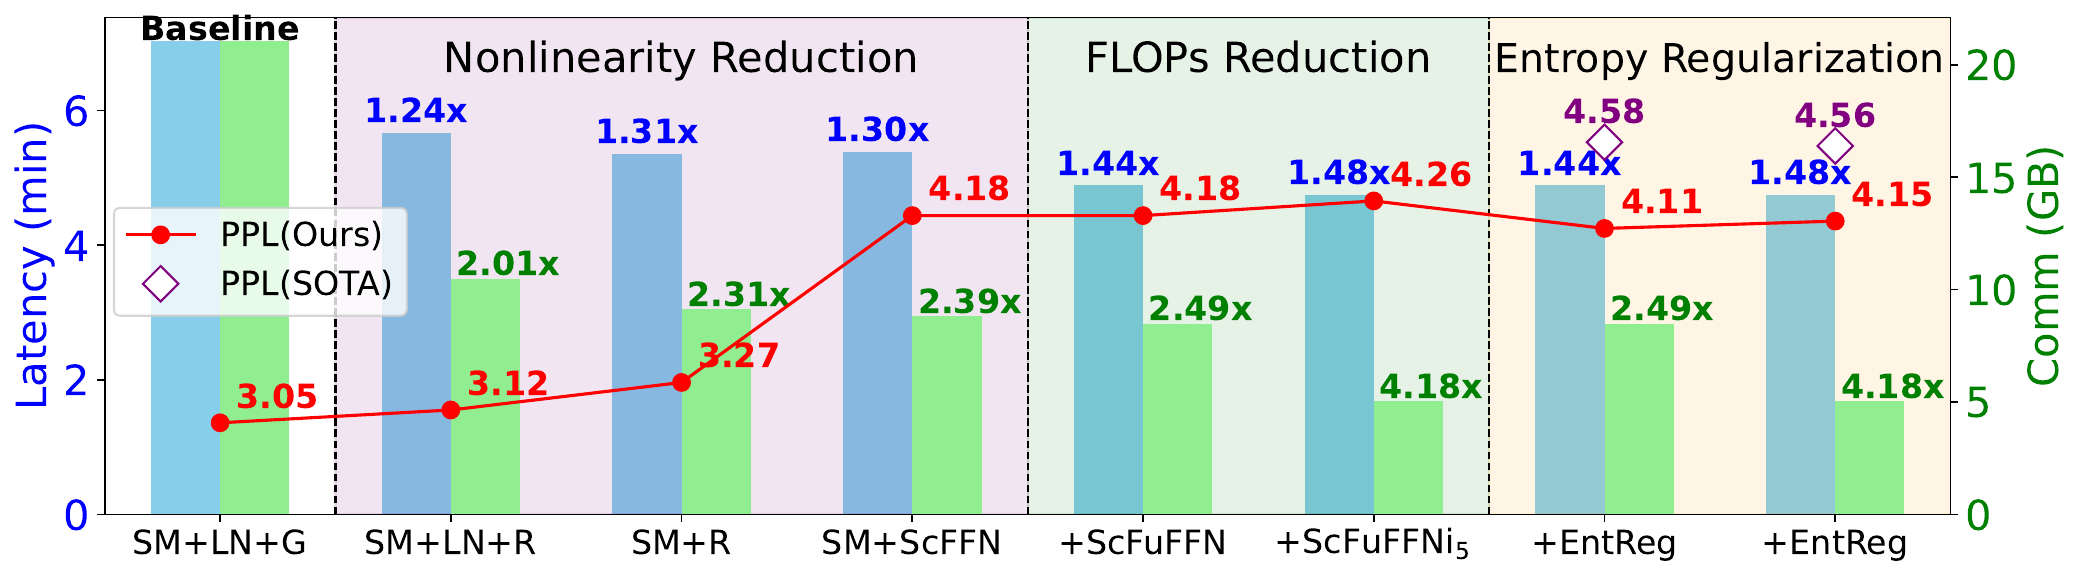} 
\caption{Latency and communication savings through nonlinearity and FLOPs reduction steps when AERO is applied on Pythia-70M, and model is trained from scratch on CodeParrot dataset with context length 256. Further, we benchmark AERO against the SOTA \cite{he2024simplifying} at iso-latency points. } 
\label{fig:PythiaVsSOTA}
\end{figure}
