# Supplementary material for: Entropy-Guided Attention for Private LLMs
Source: arXiv:2501.03489 source file (2025-01-08)
Supplement: Supplementary file 8 [file 29_fig_appendix_entropy_distribution_iFFN.tex]

\begin{wrapfigure}[18]{r}{0.65\textwidth - .95\columnsep}
\centering
\vspace{-1\intextsep}
\includegraphics[scale=0.3]{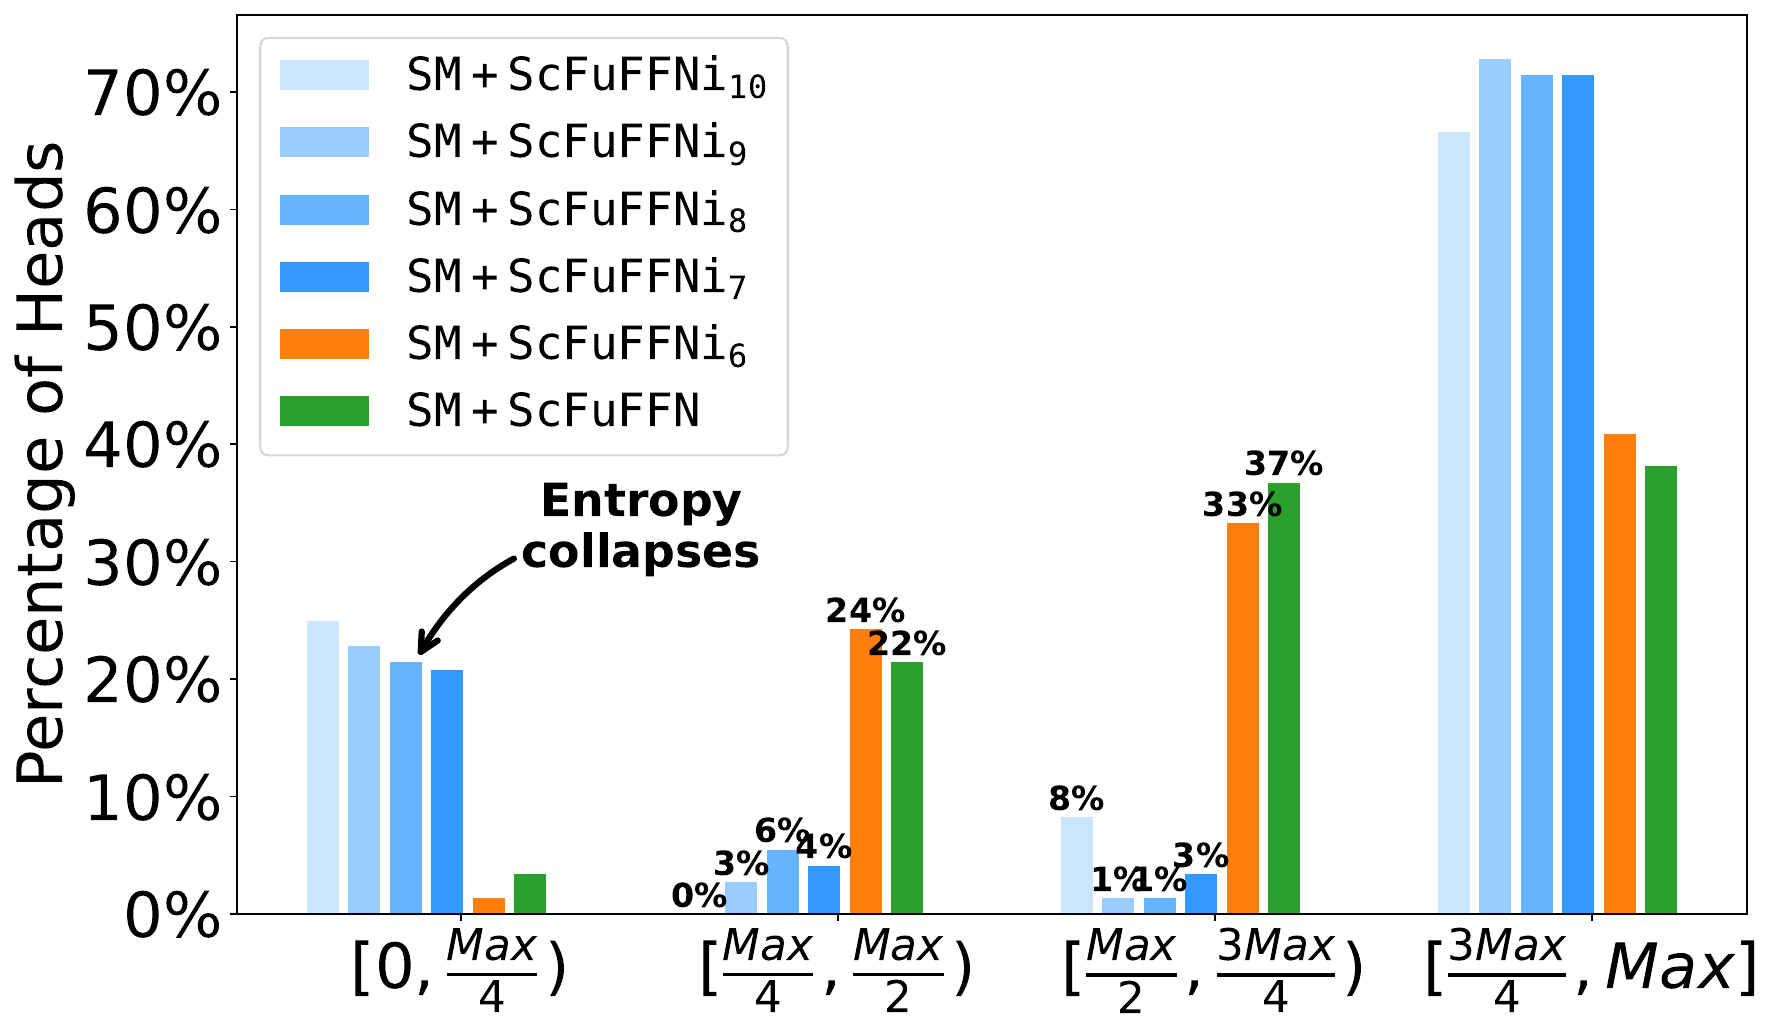} 
\vspace{-2em}
\caption{Head-wise entropy distribution in the Softmax-only GPT-2 model ($L$=12, $H$=12, $d$=768) with earlier FFNs intact and deeper FFNs pruned, trained from scratch on the CodeParrot dataset.} 
\label{fig:EntDistIdentityFFN}
\end{wrapfigure}
